# Supplementary material for: Variational Inference for Variable Selection in Scalar-on-Function Regression
Source: arXiv:2603.07856 source file (2026-03-09)
Supplement: Supplementary file 1 [file supp_sofr_realdata.tex]

\section{Additional figures for real data applications}
\label{ap:res_data}

In this section, we include the estimated partial functional coefficients obtained from the alternative methods compared in the analyses of sugar spectra and Japan weather datasets.

\begin{figure}[ht]
    \centering
    \begin{subfigure}[b]{0.27\textwidth}
        \centering
        \includegraphics[width=\textwidth, page = 1]{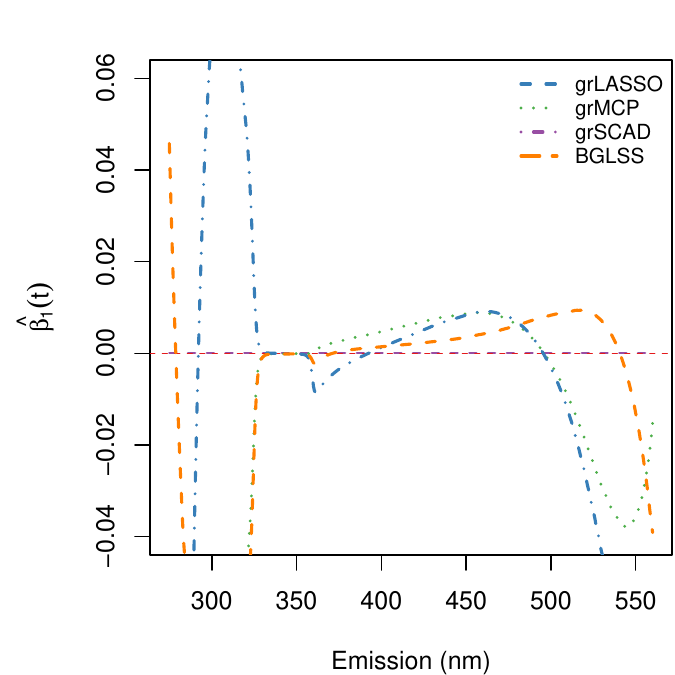}
        \caption{Excitation 230 nm}
    \end{subfigure}
    \begin{subfigure}[b]{0.27\textwidth}
        \centering
        \includegraphics[width=\textwidth, page = 2]{Comparative_results_sugar_vem.pdf}
        \caption{Excitation 240 nm}
    \end{subfigure}
    \begin{subfigure}[b]{0.27\textwidth}
        \centering
        \includegraphics[width=\textwidth, page = 3]{Comparative_results_sugar_vem.pdf}
        \caption{Excitation 255 nm}
    \end{subfigure}
     \begin{subfigure}[b]{0.27\textwidth}
        \centering
        \includegraphics[width=\textwidth, page = 4]{Comparative_results_sugar_vem.pdf}
        \caption{Excitation 290 nm}
    \end{subfigure}
     \begin{subfigure}[b]{0.27\textwidth}
        \centering
        \includegraphics[width=\textwidth, page = 5]{Comparative_results_sugar_vem.pdf}
        \caption{Excitation 305 nm}
    \end{subfigure}
     \begin{subfigure}[b]{0.27\textwidth}
        \centering
        \includegraphics[width=\textwidth, page = 6]{Comparative_results_sugar_vem.pdf}
        \caption{Excitation 325 nm}
    \end{subfigure}
     \begin{subfigure}[b]{0.27\textwidth}
        \centering
        \includegraphics[width=\textwidth, page = 7]{Comparative_results_sugar_vem.pdf}
        \caption{Excitation 340 nm}
    \end{subfigure}

    \caption[Sugar spectra dataset. Estimated functional coefficients for other methods.]{Sugar spectra dataset. The estimated curves for the functional coefficients corresponding to the seven excitation wavelengths, 230, 240, 255, 290, 305, 325, 340 nm, are shown using grLASSO (blue), grMCP (green), grSCAD (purple), and BGLSS (orange). A horizontal red line at zero is included for reference.}
    \label{fig:sugar_betas_alter}
\end{figure}

\begin{figure}[ht]
    \centering
    \begin{subfigure}[b]{0.35\textwidth}
        \centering
        \includegraphics[width=\textwidth, page = 1]{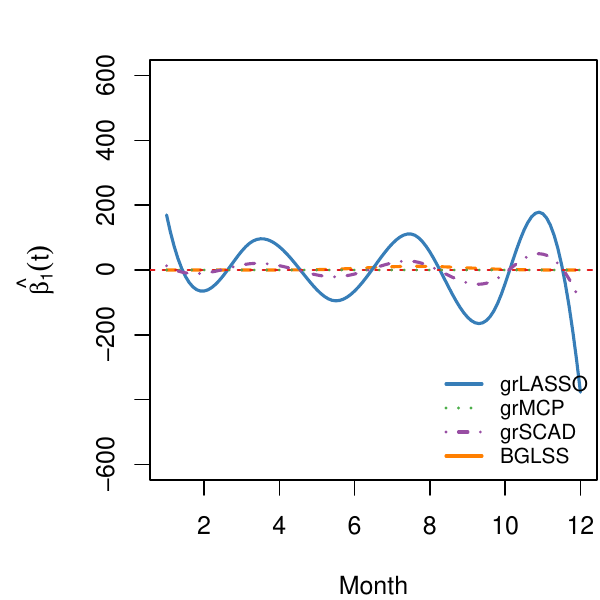}
        \caption{Temperature}
    \end{subfigure}
    \begin{subfigure}[b]{0.35\textwidth}
        \centering
        \includegraphics[width=\textwidth, page = 2]{Comparative_results_jma_vem.pdf}
        \caption{Maximum temperature}
    \end{subfigure}
    \begin{subfigure}[b]{0.35\textwidth}
        \centering
        \includegraphics[width=\textwidth, page = 3]{Comparative_results_jma_vem.pdf}
        \caption{Minimum temperature}
    \end{subfigure}
    \begin{subfigure}[b]{0.35\textwidth}
        \centering
        \includegraphics[width=\textwidth, page = 4]{Comparative_results_jma_vem.pdf}
        \caption{Pressure}
    \end{subfigure}
    \begin{subfigure}[b]{0.35\textwidth}
        \centering
        \includegraphics[width=\textwidth, page = 5]{Comparative_results_jma_vem.pdf}
        \caption{Humidity}
    \end{subfigure}
    \begin{subfigure}[b]{0.35\textwidth}
        \centering
        \includegraphics[width=\textwidth, page = 6]{Comparative_results_jma_vem.pdf}
        \caption{Daylight duration}
    \end{subfigure}

    \caption[Japan weather data. Estimated functional coefficients for other methods.]{Japan weather dataset. Estimated curves for the functional coefficients associated to the weather information for grLASSO (blue), grMCP (green), grSCAD (purple), and BGLSS (orange). A horizontal red line at zero is included for reference.}
    \label{fig:jma_betas_other}
\end{figure}
