# Supplementary material for: Variational Inference for Variable Selection in Scalar-on-Function Regression
Source: arXiv:2603.07856 source file (2026-03-09)
Supplement: Supplementary file 2 [file supp_sofr_vbpartial.tex]

\section{VEM for partially functional regression}
\label{ap:vb_partial}

In this section, we derive the VEM algorithm for partially functional regression. The proposed Bayesian hierarchical model is specified in Equation \ref{eq:hier_sofr_partial}, from which the corresponding VB update equations and the ELBO are derived. The proposed Bayesian hierarchical model for partially functional regression is given as
\begin{align}
\label{eq:hier_sofr_partial}
Y_i \mid \mathbf{Z}, \mathbf{u},\boldsymbol{\beta},\boldsymbol{\alpha},\sigma^2 &\sim \mathcal{N}\left(\mathbf{x}^S_i U \boldsymbol{\alpha} + \mathbf{W}_i\trp\Gamma\mathbf{b}, \sigma^2\right);
\nonumber\\
b_{kj} \mid \sigma^2, \tau_{kj}^2 &\sim \mathcal{N}(0, \tau_{kj}^2\sigma^2);
\nonumber\\
\alpha_{l} \mid \sigma^2, \nu_{l}^2 &\sim \mathcal{N}(0, \nu_{l}^2\sigma^2);
\nonumber\\
Z_{j} \mid \boldsymbol{\theta}_z &\sim \mathrm{Bernoulli}(\theta_{z_j});
\nonumber\\
u_{l} \mid \boldsymbol{\theta}_u &\sim \mathrm{Bernoulli}(\theta_{u_l});
\nonumber\\
\theta_{z_j} &\sim \mathrm{Beta}(0.5,0.5);
\\
\theta_{u_l} &\sim \mathrm{Beta}(0.5,0.5);
\nonumber\\
\tau_{kj}^2 &\sim \mathrm{Exponential}\left(\frac{\lambda_{b j}^2}{2}\right);
\nonumber\\
\nu_{l}^2 &\sim \mathrm{Exponential}\left(\frac{\lambda_{\alpha l}^2}{2}\right);
\nonumber\\
\sigma^2 &\sim \mbox{Inverse-Gamma}(\delta_1, \delta_2).
\nonumber
\end{align}
Based on the proposed hierarchical Bayesian model in \eqref{eq:hier_sofr_partial}, we derive the update equations for $(\mathbf{b}, \boldsymbol{\alpha}, \boldsymbol{\theta}_u, \mathbf{u}, \sigma^2, \boldsymbol{\nu}^2)$. The update equations for the other parameters are unchanged from those presented in Section \ref{sec:vb_sofr} in the main text, aside from minor notational adjustments to distinguish the parameters associated with $\mathbf{u}$ and $\mathbf{Z}$. Similarly, the expectations are computed as in Appendix \ref{sec:vb_exp_sofr} of the main text, with only minor modifications in notation. Throughout, we use $\upc$ to denote equality up to an additive constant.

The complete data-likelihood for the proposed method for partially functional regression is given as
\begin{align}
\label{eq:vb_complete_sofr_partial}
&\ p(\vec{Y}, \mathbf{Z}, \mathbf{b}, \mathbf{u}, \boldsymbol{\alpha}, \boldsymbol{\theta}_z, \boldsymbol{\theta}_u, \boldsymbol{\tau}^2,  \boldsymbol{\nu}^2, \sigma^2, \boldsymbol{\lambda}_\alpha^2, \boldsymbol{\lambda}_b^2) =
\\
=&\ p(\vec{Y} \mid \boldsymbol{\alpha}, \mathbf{b},  \mathbf{Z}, \mathbf{u},\sigma^2) \times p(\mathbf{Z} \mid \boldsymbol{\theta}_z) \times p(\mathbf{u} \mid \boldsymbol{\theta}_u) \times p(\mathbf{b} \mid \boldsymbol{\tau}^2, \sigma^2) \times p(\boldsymbol{\alpha} \mid \boldsymbol{\nu}^2, \sigma^2)
\nonumber\\
& {} \times p(\boldsymbol{\theta}_z) \times p(\boldsymbol{\theta}_u) \times p(\sigma^2) \times p(\boldsymbol{\tau}^2 \mid \boldsymbol{\lambda}_b^2) \times p(\boldsymbol{\nu}^2 \mid \boldsymbol{\lambda}_\alpha^2).
\nonumber
\end{align}

\paragraph{• Update equation for $\vec{\alpha}$:}

\begin{align*}
\log q(\vec\alpha)
=&\ \E_{q(-\vec\alpha)}(\log p(\vec{Y}, \mathbf{Z}, \mathbf{b}, \mathbf{u}, \boldsymbol{\alpha}, \boldsymbol{\theta}_z, \boldsymbol{\theta}_u, \boldsymbol{\tau}^2,  \boldsymbol{\nu}^2, \sigma^2, \boldsymbol{\lambda}_\alpha^2, \boldsymbol{\lambda}_b^2)) + \text{constant}
\\
\upc&\ \E_{q(-\vec\alpha)}\left[\log p(\vec{Y} \mid \vec\alpha, \vec{b}, \vec{u}, \vec{Z}, \sigma^2)\right] + \E_{q(-\vec\alpha)}\left[\log p(\vec\alpha \mid \vec\nu^2, \sigma^2)\right]
\\
=&\ \E_{q(-\vec\alpha)}\left[-\frac{n}{2} \log 2\pi - \frac{n}{2} \log\sigma^2 \right.\\
& {} - \left.  \frac{1}{2}\left(\frac{1}{\sigma^2}\right) \left\{\left(\vec{Y} - (X^S U \vec\alpha + W\Gamma\vec{b})\right)^\prime (\vec{Y} - (X^S U \vec\alpha + W\Gamma\vec{b}))\right\}\right]
\\
& {} + \E_{q(-\vec\alpha)}\left[ -\frac{q}{2} \log2\pi - \frac{1}{2} \log\left|I\vec\nu \sigma^2\right| - \frac{1}{2\sigma^2} \vec\alpha^\prime \diag(\vec\nu^{-1})\vec\alpha \right].
\end{align*}
Completing the squares with respect to $\boldsymbol{\alpha}$, we obtain that
\begin{align*}
& -\frac{1}{2} \frac{1}{\sigma^2} \left\{ \vec\alpha^\prime \left( \diag(\vec\nu^{-1}) + UX^{S\prime}X^SU \right) \vec\alpha
- 2 \left[ \left( \vec{Y}^\prime X^SU - \vec{b}^\prime \Gamma W^\prime X^SU \right) \vec\alpha\right]
\right\}
\\
=& -\frac{1}{2}\frac{1}{\sigma^2} \left( \vec\alpha^\prime M \vec\alpha - 2 \vec{a}^\prime \vec\alpha \right)
\\
=& -\frac{1}{2}\frac{1}{\sigma^2} \left( \left( \vec\alpha - M^{-1} \vec{a} \right)^\prime M \left( \vec\alpha - M^{-1}M \vec{a} \right) - \vec{a}^\prime M^{-1}\vec{a} \right),
\end{align*}
where $M = \diag(\vec\nu^{-1}) + UX^{S\prime}X^SU$ and $\vec{a} =  \left( \vec{Y}^\prime X^SU - \vec{b}^\prime \Gamma W^\prime X^SU \right)\trp$.

Thus, $q(\alpha)$ is a multivariate normal with
\begin{align*}
\Sigma_{\vec\alpha} &= \left( \E \left( \frac{1}{\sigma^2} \right) \left( \E \diag \left( \vec{\nu}^{-1} \right) + \E \left(  UX^{S\prime}X^SU \right) \right) \right)^{-1}
\\
\intertext{and}
\vec\mu_{\vec\alpha} &= M^{-1} \left( \E U X^{S\prime} \left( \vec{Y} - W \E(\Gamma)\E(\vec{b}) \right) \right).
\end{align*}

\paragraph{• Update equation for $\sigma^2$:}

\begin{align*}
\log q(\sigma^2)
=& \E_{q(-\sigma^2)} \left( \log p \left( \vec{Y} \mid \vec{b}, \mathbf{u}, Z, \vec\alpha, \sigma^2 \right) \right)
+ \E_{q(-\sigma^2)} \left( \log p \left( \vec{b} \mid \vec\tau^2, \sigma^2 \right) \right)
\\
&+ \E_{q(-\sigma^2)} \left( \log p \left( \vec\alpha \mid \vec\nu^2, \sigma^2 \right) \right)
+ \E_{q(-\sigma^2)} \log p \left( \sigma^2 \right)
+ \text{constant}
\\
\overset{+}{\approx} & \E_{q(-\sigma^2)} \left\{
-\frac{n}{2} \log \sigma^2 - \frac{1}{2} \frac{1}{\sigma^2} \left[ \left( \vec{Y} - \left( X^S U \vec\alpha + W \Gamma \vec{b} \right) \right)^\prime \left( \vec{Y} - \left( X^S U \vec\alpha + W \Gamma \vec{b} \right) \right) \right] \right.
\\
&\left. - \frac{K p}{2} \log \sigma^2 - \frac{1}{2 \sigma^2} \left[ \left( \vec{b}^\prime \diag (\vec{\eta}) \vec{b} \right) \right] \right.
\\
& \left. - \frac{q}{2} \log \sigma^2 - \frac{1}{2 \sigma^2} \left[ \left( \vec\alpha^\prime \diag \left( \vec\nu^{-1} \right) \vec\alpha \right) \right]
+ \left( \delta_1 + 1 \right) \log \left(\frac{1}{\sigma^2} \right) - \delta_2 \frac{1}{\sigma^2}
\right\}
\\
=& - \left( \frac{n + K p + q}{2} + \delta_1 + 1 \right) \log \sigma_2
- \frac{1}{\sigma^2} \times \frac{1}{2} \left( \E \left[ \left( \vec{Y} - \left( X^S U \vec\alpha + W \Gamma \vec{b} \right) \right)^\prime \right. \right.
\\
& \left. \left. \left( \vec{Y} - \left( X^S U \vec\alpha + W \Gamma \vec{b} \right) \right) \right]
+ \E \left( \vec{b}^\prime \diag (\vec{\eta}) \vec{b} \right) + \E \left( \vec\alpha^\prime \diag \left( \vec\nu^{-1} \right) \vec\alpha \right)
+ 2 \delta_2
\right)
\\
=& - \delta_1^* \log \sigma_2 - \frac{1}{\sigma^2} \times \delta_2^*.
\end{align*}
Thus,
$q(\sigma^2)$ is an inverse-gamma$\left( \delta_1^*, \delta_2^* \right).$

\paragraph{• Update equation for $\nu_l^2$:}

\begin{align*}
\log q \left( \nu_l^2 \right)
=& \E_{q \left( -\nu_l^2 \right)} \log p \left( \alpha_l \mid \sigma^2, \nu_l^2 \right) + \E_{q \left( -\nu_l^2 \right)} \log \left( \nu_l^2 \mid {\lambda}_{\alpha_l}^2\right) + \text{constant}
\\
=& \E_{q \left( -\nu_l^2 \right)} \left[ - \frac{1}{2} \log 2 \pi - \frac{1}{2} \log \sigma^2 - \frac{1}{2} \log \nu_l^2 - \frac{1}{2} \frac{1}{\sigma^2} \frac{1}{\nu_l^2} \alpha_l^2 \right]
\\
&+ \E_{q \left( -\nu_l^2 \right)} \left[ \log \left( \frac{\lambda_{\alpha_l}^2}{2} \right) - \frac{\lambda_{\alpha_l}^2}{2} \nu_l^2 \right]
\\
\overset{+}{\approx}& - \frac{1}{2} \log \nu_l^2 - \frac{1}{2} \left[ \E (\alpha_l^2) \E \left( \frac{1}{\sigma^2} \right) \frac{1}{\nu_l^2} + \lambda_{\alpha_l}^2\nu_{\alpha_l}^2 \right].
\end{align*}
Thus, $q \left( \nu_l^2 \right)$ is generalized-inverse-Gaussian (GIG)$\left( \frac{1}{2}, \chi_l^\alpha, \psi_l^\alpha \right)$, with
\begin{align*}
\chi_l^\alpha &= \E (\alpha_l^2) \E \left( \frac{1}{\sigma^2} \right),
\\
\psi_l^\alpha &=  \lambda_{\alpha_l}^2.
\end{align*}

\paragraph{• Update equation for $\theta_{u_l}$:}

\begin{align*}
\log q \left( \theta_{u_l} \right)
=&\ \E_{q \left( - \theta_{u_l} \right)} \left[ \log p \left( \theta_{u_l} \right) \right] + \E_{q \left( - \theta_{u_l} \right)} \left[ \log p \left( u_l \mid \theta_{u_l} \right) \right] + \text{constant}
\\
\overset{+}{\approx}&\ (0.5 - 1) \log \left( \theta_{u_l} \right) + (0.5 - 1) \log \left( 1 - \theta_{u_l} \right)
\\
& {} + \E (u_l) \log \theta_{u_l} + \left( 1 - \E (u_l) \right) \log \left( 1 - \theta_{u_l} \right)
\\
\overset{+}{\approx}&\ \left( 0.5 + \E (u_l) - 1 \right) \log \theta_{u_l} + \left( 0.5 + 1 - \E (u_l) - 1 \right) \log 1 - \theta_{u_l}.
\end{align*}
Therefore, $q \left( \theta_{u_l} \right)$ is a Beta$\left( 0.5 + \E (u_l), 1 - \E (u_l) + 0.5 \right)$

\paragraph{• Update equation for ${u_l}$:}

\begin{align*}
\log q \left( u_l \right)
=& \E_{q \left( -u_l \right)} \left[ \log p \left( \vec{Y} \mid \vec{\alpha}, \vec{b}, \vec{u}, \vec{Z}, \sigma^2 \right) \right] + \E_{q \left( -u_l \right)} \left[ \log p \left( u_l \mid \theta_{u_l} \right) \right] + \text{constant}
\\
\upc &\sum_{r = 0}^1 I \left( u_l = r \right) \left\{
- \frac{n}{2} \log 2 \pi - \frac{n}{2} \E (\log \sigma^2) \right.
\\
&  {} - \frac{1}{2} \E \left( \frac{1}{\sigma^2} \right) \E \left( \left[ \vec{Y} - \left( X^S U \vec\alpha + W \Gamma \vec{b} \right) \right]^\prime \left[ \vec{Y} - \left( X^S U \vec\alpha + W \Gamma \vec{b} \right) \right] \right)
\\
& + r \E \left( \log \theta_{u_l} \right) + (1 - r) \E \left( \log \left(1 - \theta_{u_l} \right) \right)
\Big\},
\end{align*}
where $U = \diag (\vec{u})$, $\vec{u} = \left( u_1, \dotsc, u_{l-1}, r, u_{l+1}, \dotsc, u_q \right)$.

Thus,
$q \left( u_l \right)$ is a Bernoulli$\left( p_{u_l} \right)$
\begin{align*}
p_{u_l} &= \frac{\exp \left( s_{l1} \right)}{\sum_{r=0}^1 \exp \left( s_{lr} \right)},
\end{align*}
\begin{align*}
s_{lr} = \Big\{
&- \frac{n}{2} \log 2 \pi - \frac{n}{2} \E (\log \sigma^2)
\\
&  {} - \frac{1}{2} \E \left( \frac{1}{\sigma^2} \right) \E \left( \left[ \vec{Y} - \left( X^S U \vec\alpha + W \Gamma \vec{b} \right) \right]^\prime \left[ \vec{Y} - \left( X^S U \vec\alpha + W \Gamma \vec{b} \right) \right] \right)
\\
& + r \E \left( \log \theta_{u_l} \right) + (1 - r) \E \left( \log \left(1 - \theta_{u_l} \right) \right)
\Big\}.
\end{align*}

\paragraph{• Update equation for $q \left( \vec{b} \right)$ :}

\begin{align*}
\log q \left( \vec{b} \right)
&= \E_{q \left( -\vec{b} \right)} \left( \log p \left( \vec{Y} \mid \vec{u}, \vec{Z}, \vec{b}, \vec\alpha, \sigma^2 \right) \right)
+ \E_{q \left( -\vec{b} \right)} \left( \log p \left( \vec{b} \mid \vec\tau^2, \sigma^2 \right) \right)
+ \text{constant}
\\
\overset{+}{\approx} & \E_{q \left( -\vec{b} \right)} \left\{ - \frac{1}{2 \sigma^2} \left( \vec{Y} - X^S U \vec\alpha - W \Gamma \vec{b} \right)^\prime \left( \vec{Y} - X^S U \vec\alpha - W \Gamma \vec{b} \right) \right\}
\\
&+ \E_{q \left( -\vec{b} \right)} \left\{ - \frac{\vec{b}^\prime \left( \diag \left( \vec\eta \right) \right) \vec{b}}{2 \sigma^2} \right\}.
\end{align*}
Completing the squares with respect to $\vec{b}$, we obtain that
$q \left( \vec{b} \right)$ is a MVN$(\mu_{\vec{b}}, \Sigma_{\vec{b}})$
\begin{align*}
\Sigma_{\vec{b}} &= \left( \E \left( \frac{1}{\sigma^2} \right) Q \right)^{-1},
\\
\mu_{\vec{b}} &= \left( Q^{-1} \left( \E (\Gamma) W^\prime \left( \vec{Y} - X^S \E (U) \E (\vec\alpha) \right) \right) \right),
\end{align*}
where $Q = \E \diag \vec\eta + \E \Gamma W^\prime W \Gamma$.

\subsection{Evidence Lower Bound (ELBO)}

Using the decomposition of the complete-data likelihood given in \eqref{eq:vb_complete_sofr_partial} and the mean-field variational family assumption, we derive the ELBO for the proposed VEM algorithm for the partially functional regression model. Specifically, we present the additional terms not included in Appendix \ref{sec:elbo_sofr} of the main text, which are given by
\begin{equation*}
\diff \vec\alpha = \E_{q^*}(\log p(\vec\alpha \mid  \boldsymbol{\nu}^2, \sigma^2)) -  \E_{q^*}(\log q(\vec\alpha)),
\end{equation*}
where
\begin{align*}
\E \log p \left( \vec\alpha \mid \vec\nu^2, \sigma^2 \right)
=&\ \E \left( \log \left( \prod_{l=1}^q p \left( \alpha_l \mid \nu_l^2, \sigma^2 \right) \right) \right)
\\
=&\ \E \left( \log \left( \prod_{l=1}^q \left( 2 \pi \sigma^2 \nu_l^2 \right)^{-1} \exp \left\{ - \frac{\alpha_l^2}{2 \sigma^2 \nu_l^2} \right\} \right) \right)
\\
=&\ \E \left( \sum_{l=1}^q - \frac{1}{2} \left[ \log 2 \pi + \log \sigma^2 + \log \nu_l^2 \right] - \frac{\alpha_l^2}{2 \sigma^2 \nu_l^2}\right)
\\
=&\ - \frac{q}{2} \log 2 \pi - \frac{q}{2} \E \left( \log \sigma^2 \right) - \frac{1}{2} \sum_{l=1}^q \E \left( \log \nu_l^2 \right)
\\
& {} - \frac{1}{2} \E \left( \frac{1}{\sigma^2} \right) \sum_{l=1}^q \E \left( \frac{1}{\nu_l^2} \right) \E \left( \alpha_l^2 \right).
\end{align*}
and
\begin{align*}
\E \log q (\vec\alpha)
&= \frac{q}{2} \log 2 \pi - \frac{1}{2} \log \det(\Sigma_{\vec{\alpha}}) - \frac{1}{2} \E \left((\vec{\alpha} - \mu_{\vec\alpha})\trp(\Sigma_{\vec{\alpha}})^{-1}(\vec{\alpha} - \mu_{\vec\alpha})\right)\\
& = \frac{q}{2} \log 2 \pi - \frac{1}{2} \log \det(\Sigma_{\vec{\alpha}}) - \frac{q}{2}.
\end{align*}
Thus,
\begin{align*}
\diff \vec\alpha =&\ \frac{q}{2} \E \left( \log \sigma^2 \right) - \frac{1}{2} \sum_{l=1}^q \E \left( \log \nu_l^2 \right)
\\
& {} - \frac{1}{2} \E \left( \frac{1}{\sigma^2} \right) \sum_{l=1}^q \E \left( \frac{1}{\nu_l^2} \right) \E \left( \alpha_l^2 \right) + \frac{1}{2} \log \det(\Sigma_{\vec{\alpha}}) + \frac{q}{2}.
\end{align*}

\begin{align*}
\diff \vec{\theta}_u = \E_q \left( \log p (\vec{\theta}_u) \right) - \E_q \left( \log q (\vec{\theta}_u) \right),
\end{align*}
where
\begin{align*}
\E (\log p(\vec{\theta}_u))
=&\ 
\E_q \left( \log \left( \prod_{l=1}^q {\theta_{u_l}}^{(0.5 - 1)} (1 - \theta_{u_l})^{(0.5 - 1)} \frac{\Gamma (0.5 + 0.5)}{\Gamma (0.5) \Gamma (0.5)} \right) \right)
\\
=&\ \E_q \Big( \sum_{l=1}^q \left[ (0.5 - 1) \log \theta_{u_l} + (0.5 - 1) \log (1 - \theta_{u_l})
\right. \\
& \left. {} + \log \Gamma (0.5 + 0.5) - \log 0.5 - \log 0.5 \right] \Big),
\end{align*}
and
\begin{align*}
\E \log q (\vec{\theta}_u))
=&\ \E_q \left( \log \left( \prod_{l=1}^q {\theta_{u_l}}^{(a_u^* - 1)} {\left( 1 - \theta_{u_l} \right)}^{(b_u^* - 1)} \frac{\Gamma(a_u^* + b_u^*)}{\Gamma(a_u^*) \Gamma(b_u^*)} \right) \right)
\\
=&\ \E_q \left( \sum_{l=1}^q (a_u^* - 1) \log \theta_l^* + (b_u^* - 1) \log (1 - \theta_{u_l})
\right. \\
& \left. {} + \log \Gamma(a_u^* + b_u^*) - \log a_u^* - \log b_u^* \right).
\end{align*}

Thus,
\begin{align*}
\diff \vec{\theta}_u
=& \sum_{l=1}^q \Big( (0.5 - 1) \E \log \theta_{u_l} + (0.5 - 1) \E \log (1 - \theta_{u_l})
\\
& - 2\log 0.5 - (a_{u_l}^* - 1) \E \log \theta_{u_l} - (b_{u_l}^* - 1) \E \log (1 - \theta_{u_l})
\\
& - \log \Gamma ( a_{u_l}^* + b_{u_l}^* ) + \log \Gamma a_{u_l}^* + \log \Gamma b_{u_l}^* \Big)
\end{align*}
\begin{align*}
\diff \vec\nu^2 = \E_q \left( \log p (\vec\nu^2 \right) - \E_q \left( \log q (\vec\nu^2) \right),
\end{align*}
where
\begin{align*}
\E \log p (\vec\nu^2)
=& \E \left( \log \prod_{l=1}^q \left( \frac{\lambda_{\alpha l}^2}{2} \exp \left( - \frac{\lambda_{\alpha l}^2}{2} \nu_l^2 \right) \right) \right)
\\
=& \E \left( \sum_{l=1}^q \left( \log \lambda_{\alpha l}^2 - \log 2 -  \frac{\lambda_{\alpha l}^2}{2} \nu_l^2 \right) \right)
\end{align*}
and
\begin{align*}
\E \log q (\vec\nu^2)
=& \E \left( \log \prod_{l=1}^q \left( \frac{\left( \frac{\psi_{\alpha_l}}{\chi_{\alpha_l}} \right)^{\frac{1}{4}}}{2 K_{1/2} \sqrt{\psi_{\alpha_l} \chi_{\alpha_l}}} \right) \right.
\\
& \left. (\nu_l^2)^{(0.5 - 1)} \exp \left\{ \frac{- \psi_{\alpha_l} \nu_l^2 + \frac{\chi_{\alpha_l}}{\nu_l^2}}{2} \right\} \right)
\\
=& \sum_{l=1}^q \frac{1}{4} \left[ \log (\psi_{\alpha_l}) - \log (\chi_{\alpha_l})  \right] - \log \left( 2 K_{1/2} \sqrt{\psi_{\alpha_l} \chi_{\alpha_l}} \right)
\\
& + (0.5 - 1) \E \log \nu_l^2 - \frac{1}{2} \left( \psi_{\alpha_l} \E \nu_l^2 +  \chi_{\alpha_l} \E \left( \frac{1}{\nu_l^2} \right) \right).
\end{align*}

Thus,
\begin{align*}
\diff \vec\nu^2
=& \sum_{l=1}^q \left( \log \lambda_{\alpha_l}^2 - \frac{\lambda_{\alpha_l}^2}{2} \E (\nu_l^2) \right.
\\
&  - \frac{1}{4} \left[ \log \psi_{\alpha_l} + \log \chi_{\alpha_l} \right] + \log \left( K_{1/2} \sqrt{\psi_{\alpha_l} \chi_{\alpha_l}} \right)
\\
& \left. - (0.5 - 1) \E \log (\nu_l^2) + \frac{1}{2} \left( \psi_{\alpha_l} \E (\nu_l^2) + \chi_{\alpha_l} \E \frac{1}{\nu_l^2} \right) \right).
\end{align*}
