# Supplementary material for: Variational Inference for Variable Selection in Scalar-on-Function Regression
Source: arXiv:2603.07856 source file (2026-03-09)
Supplement: Supplementary file 3 [file Supplementary_material.tex]

\documentclass[12pt]{article}

\usepackage[margin=1in]{geometry}

% Useful packages
\usepackage{amsmath}
\usepackage{amssymb}
\usepackage{graphicx}
\usepackage{booktabs}

\usepackage{hyperref}
\usepackage{xr}
\externaldocument{main}

\usepackage{natbib}

\usepackage{subcaption}

\usepackage{algorithm}
\usepackage{algpseudocode}

\DeclareMathOperator{\E}{E}

\DeclareMathOperator*{\upc}{\overset{+}{\approx}}
\DeclareMathOperator{\diag}{diag}

\DeclareMathOperator{\diff}{diff}

\newcommand{\trp}{^{\prime}}

\renewcommand{\vec}[1]{\boldsymbol{#1}}

\title{Variational Inference for Variable Selection in Scalar-on-Function Regression \\
Supplementary Material}
\author{Ana Carolina da Cruz$^{1*}$ \and \ Camila P.\ E.\ de Souza$^1$ \and \ Pedro H.\ T.\ O.\ Sousa$^2$ \\  
\normalsize $^1$Department of Statistical and Actuarial Sciences, University of Western Ontario, Canada\\
\normalsize $^2$Department of Statistics, Federal University of Paraná, Brazil \\
\normalsize$^*$Corresponding author: adacruz@uwo.ca}
\date{}

\begin{document}
\maketitle

\section{VEM for partially functional regression}
\label{ap:vb_partial}

In this section, we derive the VEM algorithm for partially functional regression. The proposed Bayesian hierarchical model is specified in Equation \ref{eq:hier_sofr_partial}, from which the corresponding VB update equations and the ELBO are derived. The proposed Bayesian hierarchical model for partially functional regression is given as
\begin{align}
\label{eq:hier_sofr_partial}
Y_i \mid \mathbf{Z}, \mathbf{u},\boldsymbol{\beta},\boldsymbol{\alpha},\sigma^2 &\sim \mathcal{N}\left(\mathbf{x}^S_i U \boldsymbol{\alpha} + \mathbf{W}_i\trp\Gamma\mathbf{b}, \sigma^2\right);
\nonumber\\
b_{kj} \mid \sigma^2, \tau_{kj}^2 &\sim \mathcal{N}(0, \tau_{kj}^2\sigma^2);
\nonumber\\
\alpha_{l} \mid \sigma^2, \nu_{l}^2 &\sim \mathcal{N}(0, \nu_{l}^2\sigma^2);
\nonumber\\
Z_{j} \mid \boldsymbol{\theta}_z &\sim \mathrm{Bernoulli}(\theta_{z_j});
\nonumber\\
u_{l} \mid \boldsymbol{\theta}_u &\sim \mathrm{Bernoulli}(\theta_{u_l});
\nonumber\\
\theta_{z_j} &\sim \mathrm{Beta}(0.5,0.5);
\\
\theta_{u_l} &\sim \mathrm{Beta}(0.5,0.5);
\nonumber\\
\tau_{kj}^2 &\sim \mathrm{Exponential}\left(\frac{\lambda_{b j}^2}{2}\right);
\nonumber\\
\nu_{l}^2 &\sim \mathrm{Exponential}\left(\frac{\lambda_{\alpha l}^2}{2}\right);
\nonumber\\
\sigma^2 &\sim \mbox{Inverse-Gamma}(\delta_1, \delta_2).
\nonumber
\end{align}
Based on the proposed hierarchical Bayesian model in \eqref{eq:hier_sofr_partial}, we derive the update equations for $(\mathbf{b}, \boldsymbol{\alpha}, \boldsymbol{\theta}_u, \mathbf{u}, \sigma^2, \boldsymbol{\nu}^2)$. The update equations for the other parameters are unchanged from those presented in Section \ref{sec:vb_sofr} in the main text, aside from minor notational adjustments to distinguish the parameters associated with $\mathbf{u}$ and $\mathbf{Z}$. Similarly, the expectations are computed as in Appendix \ref{sec:vb_exp_sofr} of the main text, with only minor modifications in notation. Throughout, we use $\upc$ to denote equality up to an additive constant.

The complete data-likelihood for the proposed method for partially functional regression is given as
\begin{align}
\label{eq:vb_complete_sofr_partial}
&\ p(\vec{Y}, \mathbf{Z}, \mathbf{b}, \mathbf{u}, \boldsymbol{\alpha}, \boldsymbol{\theta}_z, \boldsymbol{\theta}_u, \boldsymbol{\tau}^2,  \boldsymbol{\nu}^2, \sigma^2, \boldsymbol{\lambda}_\alpha^2, \boldsymbol{\lambda}_b^2) =
\\
=&\ p(\vec{Y} \mid \boldsymbol{\alpha}, \mathbf{b},  \mathbf{Z}, \mathbf{u},\sigma^2) \times p(\mathbf{Z} \mid \boldsymbol{\theta}_z) \times p(\mathbf{u} \mid \boldsymbol{\theta}_u) \times p(\mathbf{b} \mid \boldsymbol{\tau}^2, \sigma^2) \times p(\boldsymbol{\alpha} \mid \boldsymbol{\nu}^2, \sigma^2)
\nonumber\\
& {} \times p(\boldsymbol{\theta}_z) \times p(\boldsymbol{\theta}_u) \times p(\sigma^2) \times p(\boldsymbol{\tau}^2 \mid \boldsymbol{\lambda}_b^2) \times p(\boldsymbol{\nu}^2 \mid \boldsymbol{\lambda}_\alpha^2).
\nonumber
\end{align}

\paragraph{• Update equation for $\vec{\alpha}$:}

\begin{align*}
\log q(\vec\alpha)
=&\ \E_{q(-\vec\alpha)}(\log p(\vec{Y}, \mathbf{Z}, \mathbf{b}, \mathbf{u}, \boldsymbol{\alpha}, \boldsymbol{\theta}_z, \boldsymbol{\theta}_u, \boldsymbol{\tau}^2,  \boldsymbol{\nu}^2, \sigma^2, \boldsymbol{\lambda}_\alpha^2, \boldsymbol{\lambda}_b^2)) + \text{constant}
\\
\upc&\ \E_{q(-\vec\alpha)}\left[\log p(\vec{Y} \mid \vec\alpha, \vec{b}, \vec{u}, \vec{Z}, \sigma^2)\right] + \E_{q(-\vec\alpha)}\left[\log p(\vec\alpha \mid \vec\nu^2, \sigma^2)\right]
\\
=&\ \E_{q(-\vec\alpha)}\left[-\frac{n}{2} \log 2\pi - \frac{n}{2} \log\sigma^2 \right.\\
& {} - \left.  \frac{1}{2}\left(\frac{1}{\sigma^2}\right) \left\{\left(\vec{Y} - (X^S U \vec\alpha + W\Gamma\vec{b})\right)^\prime (\vec{Y} - (X^S U \vec\alpha + W\Gamma\vec{b}))\right\}\right]
\\
& {} + \E_{q(-\vec\alpha)}\left[ -\frac{q}{2} \log2\pi - \frac{1}{2} \log\left|I\vec\nu \sigma^2\right| - \frac{1}{2\sigma^2} \vec\alpha^\prime \diag(\vec\nu^{-1})\vec\alpha \right].
\end{align*}
Completing the squares with respect to $\boldsymbol{\alpha}$, we obtain that
\begin{align*}
& -\frac{1}{2} \frac{1}{\sigma^2} \left\{ \vec\alpha^\prime \left( \diag(\vec\nu^{-1}) + UX^{S\prime}X^SU \right) \vec\alpha
- 2 \left[ \left( \vec{Y}^\prime X^SU - \vec{b}^\prime \Gamma W^\prime X^SU \right) \vec\alpha\right]
\right\}
\\
=& -\frac{1}{2}\frac{1}{\sigma^2} \left( \vec\alpha^\prime M \vec\alpha - 2 \vec{a}^\prime \vec\alpha \right)
\\
=& -\frac{1}{2}\frac{1}{\sigma^2} \left( \left( \vec\alpha - M^{-1} \vec{a} \right)^\prime M \left( \vec\alpha - M^{-1}M \vec{a} \right) - \vec{a}^\prime M^{-1}\vec{a} \right),
\end{align*}
where $M = \diag(\vec\nu^{-1}) + UX^{S\prime}X^SU$ and $\vec{a} =  \left( \vec{Y}^\prime X^SU - \vec{b}^\prime \Gamma W^\prime X^SU \right)\trp$.

Thus, $q(\alpha)$ is a multivariate normal with
\begin{align*}
\Sigma_{\vec\alpha} &= \left( \E \left( \frac{1}{\sigma^2} \right) \left( \E \diag \left( \vec{\nu}^{-1} \right) + \E \left(  UX^{S\prime}X^SU \right) \right) \right)^{-1}
\\
\intertext{and}
\vec\mu_{\vec\alpha} &= M^{-1} \left( \E U X^{S\prime} \left( \vec{Y} - W \E(\Gamma)\E(\vec{b}) \right) \right).
\end{align*}

\paragraph{• Update equation for $\sigma^2$:}

\begin{align*}
\log q(\sigma^2)
=& \E_{q(-\sigma^2)} \left( \log p \left( \vec{Y} \mid \vec{b}, \mathbf{u}, Z, \vec\alpha, \sigma^2 \right) \right)
+ \E_{q(-\sigma^2)} \left( \log p \left( \vec{b} \mid \vec\tau^2, \sigma^2 \right) \right)
\\
&+ \E_{q(-\sigma^2)} \left( \log p \left( \vec\alpha \mid \vec\nu^2, \sigma^2 \right) \right)
+ \E_{q(-\sigma^2)} \log p \left( \sigma^2 \right)
+ \text{constant}
\\
\overset{+}{\approx} & \E_{q(-\sigma^2)} \left\{
-\frac{n}{2} \log \sigma^2 - \frac{1}{2} \frac{1}{\sigma^2} \left[ \left( \vec{Y} - \left( X^S U \vec\alpha + W \Gamma \vec{b} \right) \right)^\prime \left( \vec{Y} - \left( X^S U \vec\alpha + W \Gamma \vec{b} \right) \right) \right] \right.
\\
&\left. - \frac{K p}{2} \log \sigma^2 - \frac{1}{2 \sigma^2} \left[ \left( \vec{b}^\prime \diag (\vec{\eta}) \vec{b} \right) \right] \right.
\\
& \left. - \frac{q}{2} \log \sigma^2 - \frac{1}{2 \sigma^2} \left[ \left( \vec\alpha^\prime \diag \left( \vec\nu^{-1} \right) \vec\alpha \right) \right]
+ \left( \delta_1 + 1 \right) \log \left(\frac{1}{\sigma^2} \right) - \delta_2 \frac{1}{\sigma^2}
\right\}
\\
=& - \left( \frac{n + K p + q}{2} + \delta_1 + 1 \right) \log \sigma_2
- \frac{1}{\sigma^2} \times \frac{1}{2} \left( \E \left[ \left( \vec{Y} - \left( X^S U \vec\alpha + W \Gamma \vec{b} \right) \right)^\prime \right. \right.
\\
& \left. \left. \left( \vec{Y} - \left( X^S U \vec\alpha + W \Gamma \vec{b} \right) \right) \right]
+ \E \left( \vec{b}^\prime \diag (\vec{\eta}) \vec{b} \right) + \E \left( \vec\alpha^\prime \diag \left( \vec\nu^{-1} \right) \vec\alpha \right)
+ 2 \delta_2
\right)
\\
=& - \delta_1^* \log \sigma_2 - \frac{1}{\sigma^2} \times \delta_2^*.
\end{align*}
Thus,
$q(\sigma^2)$ is an inverse-gamma$\left( \delta_1^*, \delta_2^* \right).$

\paragraph{• Update equation for $\nu_l^2$:}

\begin{align*}
\log q \left( \nu_l^2 \right)
=& \E_{q \left( -\nu_l^2 \right)} \log p \left( \alpha_l \mid \sigma^2, \nu_l^2 \right) + \E_{q \left( -\nu_l^2 \right)} \log \left( \nu_l^2 \mid {\lambda}_{\alpha_l}^2\right) + \text{constant}
\\
=& \E_{q \left( -\nu_l^2 \right)} \left[ - \frac{1}{2} \log 2 \pi - \frac{1}{2} \log \sigma^2 - \frac{1}{2} \log \nu_l^2 - \frac{1}{2} \frac{1}{\sigma^2} \frac{1}{\nu_l^2} \alpha_l^2 \right]
\\
&+ \E_{q \left( -\nu_l^2 \right)} \left[ \log \left( \frac{\lambda_{\alpha_l}^2}{2} \right) - \frac{\lambda_{\alpha_l}^2}{2} \nu_l^2 \right]
\\
\overset{+}{\approx}& - \frac{1}{2} \log \nu_l^2 - \frac{1}{2} \left[ \E (\alpha_l^2) \E \left( \frac{1}{\sigma^2} \right) \frac{1}{\nu_l^2} + \lambda_{\alpha_l}^2\nu_{\alpha_l}^2 \right].
\end{align*}
Thus, $q \left( \nu_l^2 \right)$ is generalized-inverse-Gaussian (GIG)$\left( \frac{1}{2}, \chi_l^\alpha, \psi_l^\alpha \right)$, with
\begin{align*}
\chi_l^\alpha &= \E (\alpha_l^2) \E \left( \frac{1}{\sigma^2} \right),
\\
\psi_l^\alpha &=  \lambda_{\alpha_l}^2.
\end{align*}

\paragraph{• Update equation for $\theta_{u_l}$:}

\begin{align*}
\log q \left( \theta_{u_l} \right)
=&\ \E_{q \left( - \theta_{u_l} \right)} \left[ \log p \left( \theta_{u_l} \right) \right] + \E_{q \left( - \theta_{u_l} \right)} \left[ \log p \left( u_l \mid \theta_{u_l} \right) \right] + \text{constant}
\\
\overset{+}{\approx}&\ (0.5 - 1) \log \left( \theta_{u_l} \right) + (0.5 - 1) \log \left( 1 - \theta_{u_l} \right)
\\
& {} + \E (u_l) \log \theta_{u_l} + \left( 1 - \E (u_l) \right) \log \left( 1 - \theta_{u_l} \right)
\\
\overset{+}{\approx}&\ \left( 0.5 + \E (u_l) - 1 \right) \log \theta_{u_l} + \left( 0.5 + 1 - \E (u_l) - 1 \right) \log 1 - \theta_{u_l}.
\end{align*}
Therefore, $q \left( \theta_{u_l} \right)$ is a Beta$\left( 0.5 + \E (u_l), 1 - \E (u_l) + 0.5 \right)$

\paragraph{• Update equation for ${u_l}$:}

\begin{align*}
\log q \left( u_l \right)
=& \E_{q \left( -u_l \right)} \left[ \log p \left( \vec{Y} \mid \vec{\alpha}, \vec{b}, \vec{u}, \vec{Z}, \sigma^2 \right) \right] + \E_{q \left( -u_l \right)} \left[ \log p \left( u_l \mid \theta_{u_l} \right) \right] + \text{constant}
\\
\upc &\sum_{r = 0}^1 I \left( u_l = r \right) \left\{
- \frac{n}{2} \log 2 \pi - \frac{n}{2} \E (\log \sigma^2) \right.
\\
&  {} - \frac{1}{2} \E \left( \frac{1}{\sigma^2} \right) \E \left( \left[ \vec{Y} - \left( X^S U \vec\alpha + W \Gamma \vec{b} \right) \right]^\prime \left[ \vec{Y} - \left( X^S U \vec\alpha + W \Gamma \vec{b} \right) \right] \right)
\\
& + r \E \left( \log \theta_{u_l} \right) + (1 - r) \E \left( \log \left(1 - \theta_{u_l} \right) \right)
\Big\},
\end{align*}
where $U = \diag (\vec{u})$, $\vec{u} = \left( u_1, \dotsc, u_{l-1}, r, u_{l+1}, \dotsc, u_q \right)$.

Thus,
$q \left( u_l \right)$ is a Bernoulli$\left( p_{u_l} \right)$
\begin{align*}
p_{u_l} &= \frac{\exp \left( s_{l1} \right)}{\sum_{r=0}^1 \exp \left( s_{lr} \right)},
\end{align*}
\begin{align*}
s_{lr} = \Big\{
&- \frac{n}{2} \log 2 \pi - \frac{n}{2} \E (\log \sigma^2)
\\
&  {} - \frac{1}{2} \E \left( \frac{1}{\sigma^2} \right) \E \left( \left[ \vec{Y} - \left( X^S U \vec\alpha + W \Gamma \vec{b} \right) \right]^\prime \left[ \vec{Y} - \left( X^S U \vec\alpha + W \Gamma \vec{b} \right) \right] \right)
\\
& + r \E \left( \log \theta_{u_l} \right) + (1 - r) \E \left( \log \left(1 - \theta_{u_l} \right) \right)
\Big\}.
\end{align*}

\paragraph{• Update equation for $q \left( \vec{b} \right)$ :}

\begin{align*}
\log q \left( \vec{b} \right)
&= \E_{q \left( -\vec{b} \right)} \left( \log p \left( \vec{Y} \mid \vec{u}, \vec{Z}, \vec{b}, \vec\alpha, \sigma^2 \right) \right)
+ \E_{q \left( -\vec{b} \right)} \left( \log p \left( \vec{b} \mid \vec\tau^2, \sigma^2 \right) \right)
+ \text{constant}
\\
\overset{+}{\approx} & \E_{q \left( -\vec{b} \right)} \left\{ - \frac{1}{2 \sigma^2} \left( \vec{Y} - X^S U \vec\alpha - W \Gamma \vec{b} \right)^\prime \left( \vec{Y} - X^S U \vec\alpha - W \Gamma \vec{b} \right) \right\}
\\
&+ \E_{q \left( -\vec{b} \right)} \left\{ - \frac{\vec{b}^\prime \left( \diag \left( \vec\eta \right) \right) \vec{b}}{2 \sigma^2} \right\}.
\end{align*}
Completing the squares with respect to $\vec{b}$, we obtain that
$q \left( \vec{b} \right)$ is a MVN$(\mu_{\vec{b}}, \Sigma_{\vec{b}})$
\begin{align*}
\Sigma_{\vec{b}} &= \left( \E \left( \frac{1}{\sigma^2} \right) Q \right)^{-1},
\\
\mu_{\vec{b}} &= \left( Q^{-1} \left( \E (\Gamma) W^\prime \left( \vec{Y} - X^S \E (U) \E (\vec\alpha) \right) \right) \right),
\end{align*}
where $Q = \E \diag \vec\eta + \E \Gamma W^\prime W \Gamma$.

\subsection{Evidence Lower Bound (ELBO)}

Using the decomposition of the complete-data likelihood given in \eqref{eq:vb_complete_sofr_partial} and the mean-field variational family assumption, we derive the ELBO for the proposed VEM algorithm for the partially functional regression model. Specifically, we present the additional terms not included in Appendix \ref{sec:elbo_sofr} of the main text, which are given by
\begin{equation*}
\diff \vec\alpha = \E_{q^*}(\log p(\vec\alpha \mid  \boldsymbol{\nu}^2, \sigma^2)) -  \E_{q^*}(\log q(\vec\alpha)),
\end{equation*}
where
\begin{align*}
\E \log p \left( \vec\alpha \mid \vec\nu^2, \sigma^2 \right)
=&\ \E \left( \log \left( \prod_{l=1}^q p \left( \alpha_l \mid \nu_l^2, \sigma^2 \right) \right) \right)
\\
=&\ \E \left( \log \left( \prod_{l=1}^q \left( 2 \pi \sigma^2 \nu_l^2 \right)^{-1} \exp \left\{ - \frac{\alpha_l^2}{2 \sigma^2 \nu_l^2} \right\} \right) \right)
\\
=&\ \E \left( \sum_{l=1}^q - \frac{1}{2} \left[ \log 2 \pi + \log \sigma^2 + \log \nu_l^2 \right] - \frac{\alpha_l^2}{2 \sigma^2 \nu_l^2}\right)
\\
=&\ - \frac{q}{2} \log 2 \pi - \frac{q}{2} \E \left( \log \sigma^2 \right) - \frac{1}{2} \sum_{l=1}^q \E \left( \log \nu_l^2 \right)
\\
& {} - \frac{1}{2} \E \left( \frac{1}{\sigma^2} \right) \sum_{l=1}^q \E \left( \frac{1}{\nu_l^2} \right) \E \left( \alpha_l^2 \right).
\end{align*}
and
\begin{align*}
\E \log q (\vec\alpha)
&= \frac{q}{2} \log 2 \pi - \frac{1}{2} \log \det(\Sigma_{\vec{\alpha}}) - \frac{1}{2} \E \left((\vec{\alpha} - \mu_{\vec\alpha})\trp(\Sigma_{\vec{\alpha}})^{-1}(\vec{\alpha} - \mu_{\vec\alpha})\right)\\
& = \frac{q}{2} \log 2 \pi - \frac{1}{2} \log \det(\Sigma_{\vec{\alpha}}) - \frac{q}{2}.
\end{align*}
Thus,
\begin{align*}
\diff \vec\alpha =&\ \frac{q}{2} \E \left( \log \sigma^2 \right) - \frac{1}{2} \sum_{l=1}^q \E \left( \log \nu_l^2 \right)
\\
& {} - \frac{1}{2} \E \left( \frac{1}{\sigma^2} \right) \sum_{l=1}^q \E \left( \frac{1}{\nu_l^2} \right) \E \left( \alpha_l^2 \right) + \frac{1}{2} \log \det(\Sigma_{\vec{\alpha}}) + \frac{q}{2}.
\end{align*}

\begin{align*}
\diff \vec{\theta}_u = \E_q \left( \log p (\vec{\theta}_u) \right) - \E_q \left( \log q (\vec{\theta}_u) \right),
\end{align*}
where
\begin{align*}
\E (\log p(\vec{\theta}_u))
=&\ 
\E_q \left( \log \left( \prod_{l=1}^q {\theta_{u_l}}^{(0.5 - 1)} (1 - \theta_{u_l})^{(0.5 - 1)} \frac{\Gamma (0.5 + 0.5)}{\Gamma (0.5) \Gamma (0.5)} \right) \right)
\\
=&\ \E_q \Big( \sum_{l=1}^q \left[ (0.5 - 1) \log \theta_{u_l} + (0.5 - 1) \log (1 - \theta_{u_l})
\right. \\
& \left. {} + \log \Gamma (0.5 + 0.5) - \log 0.5 - \log 0.5 \right] \Big),
\end{align*}
and
\begin{align*}
\E \log q (\vec{\theta}_u))
=&\ \E_q \left( \log \left( \prod_{l=1}^q {\theta_{u_l}}^{(a_u^* - 1)} {\left( 1 - \theta_{u_l} \right)}^{(b_u^* - 1)} \frac{\Gamma(a_u^* + b_u^*)}{\Gamma(a_u^*) \Gamma(b_u^*)} \right) \right)
\\
=&\ \E_q \left( \sum_{l=1}^q (a_u^* - 1) \log \theta_l^* + (b_u^* - 1) \log (1 - \theta_{u_l})
\right. \\
& \left. {} + \log \Gamma(a_u^* + b_u^*) - \log a_u^* - \log b_u^* \right).
\end{align*}

Thus,
\begin{align*}
\diff \vec{\theta}_u
=& \sum_{l=1}^q \Big( (0.5 - 1) \E \log \theta_{u_l} + (0.5 - 1) \E \log (1 - \theta_{u_l})
\\
& - 2\log 0.5 - (a_{u_l}^* - 1) \E \log \theta_{u_l} - (b_{u_l}^* - 1) \E \log (1 - \theta_{u_l})
\\
& - \log \Gamma ( a_{u_l}^* + b_{u_l}^* ) + \log \Gamma a_{u_l}^* + \log \Gamma b_{u_l}^* \Big)
\end{align*}
\begin{align*}
\diff \vec\nu^2 = \E_q \left( \log p (\vec\nu^2 \right) - \E_q \left( \log q (\vec\nu^2) \right),
\end{align*}
where
\begin{align*}
\E \log p (\vec\nu^2)
=& \E \left( \log \prod_{l=1}^q \left( \frac{\lambda_{\alpha l}^2}{2} \exp \left( - \frac{\lambda_{\alpha l}^2}{2} \nu_l^2 \right) \right) \right)
\\
=& \E \left( \sum_{l=1}^q \left( \log \lambda_{\alpha l}^2 - \log 2 -  \frac{\lambda_{\alpha l}^2}{2} \nu_l^2 \right) \right)
\end{align*}
and
\begin{align*}
\E \log q (\vec\nu^2)
=& \E \left( \log \prod_{l=1}^q \left( \frac{\left( \frac{\psi_{\alpha_l}}{\chi_{\alpha_l}} \right)^{\frac{1}{4}}}{2 K_{1/2} \sqrt{\psi_{\alpha_l} \chi_{\alpha_l}}} \right) \right.
\\
& \left. (\nu_l^2)^{(0.5 - 1)} \exp \left\{ \frac{- \psi_{\alpha_l} \nu_l^2 + \frac{\chi_{\alpha_l}}{\nu_l^2}}{2} \right\} \right)
\\
=& \sum_{l=1}^q \frac{1}{4} \left[ \log (\psi_{\alpha_l}) - \log (\chi_{\alpha_l})  \right] - \log \left( 2 K_{1/2} \sqrt{\psi_{\alpha_l} \chi_{\alpha_l}} \right)
\\
& + (0.5 - 1) \E \log \nu_l^2 - \frac{1}{2} \left( \psi_{\alpha_l} \E \nu_l^2 +  \chi_{\alpha_l} \E \left( \frac{1}{\nu_l^2} \right) \right).
\end{align*}

Thus,
\begin{align*}
\diff \vec\nu^2
=& \sum_{l=1}^q \left( \log \lambda_{\alpha_l}^2 - \frac{\lambda_{\alpha_l}^2}{2} \E (\nu_l^2) \right.
\\
&  - \frac{1}{4} \left[ \log \psi_{\alpha_l} + \log \chi_{\alpha_l} \right] + \log \left( K_{1/2} \sqrt{\psi_{\alpha_l} \chi_{\alpha_l}} \right)
\\
& \left. - (0.5 - 1) \E \log (\nu_l^2) + \frac{1}{2} \left( \psi_{\alpha_l} \E (\nu_l^2) + \chi_{\alpha_l} \E \frac{1}{\nu_l^2} \right) \right).
\end{align*}

\section{Additional figures for simulation studies}
\label{ap:res_sim}
\setcounter{figure}{0}

In this section, we include additional figures from the simulations studies described in the main text.

\begin{figure}[ht]
    \centering
    \begin{subfigure}[b]{\textwidth}
        \centering
        \includegraphics[width=\textwidth]{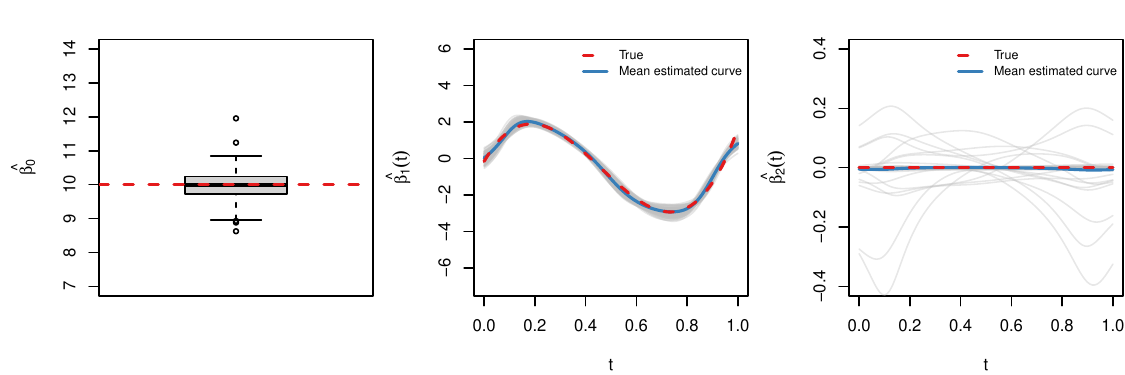}
        \caption{$\sigma^2 = 0.1$}
    \end{subfigure}
    \hfill
    \begin{subfigure}[b]{\textwidth}
        \centering
        \includegraphics[width=\textwidth]{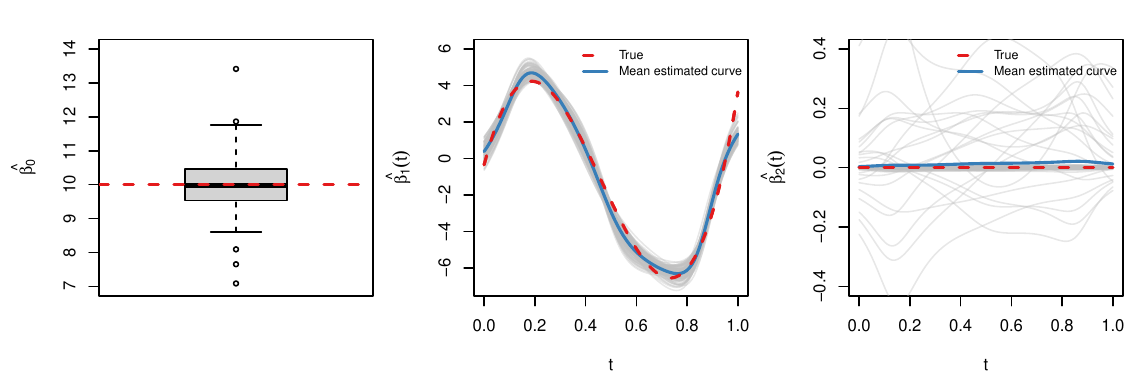}
        \caption{$\sigma^2 = 0.5$}
    \end{subfigure}

    \caption[Simulation Study 1. Estimated functional coefficients per dataset and boxplot of the intercept when $n = 50$.]{Simulation Study 1. Mean estimated curves for the two functional coefficients (blue), individual estimates per simulated dataset (grey), and boxplots of the estimated intercept across 100 simulated datasets, for sample size $n = 50$ and varying error variance ($\sigma^2 = 0.1, 0.5$). True values for the partial functional coefficients and intercept are shown in red.}
    \label{fig:sim1_all_n50_sofr}
\end{figure}

\begin{figure}[ht]
    \centering
    \begin{subfigure}[b]{\textwidth}
        \centering
        \includegraphics[width=\textwidth]{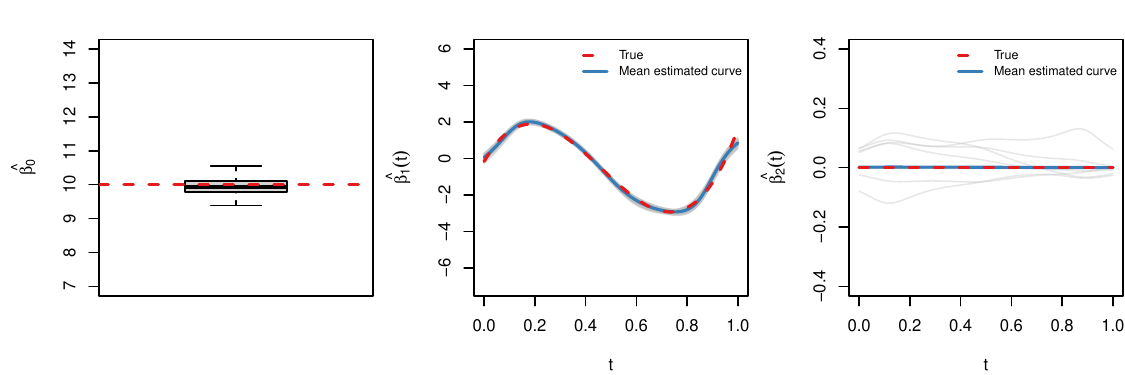}
        \caption{$\sigma^2 = 0.1$}
    \end{subfigure}
    \begin{subfigure}[b]{\textwidth}
        \centering
        \includegraphics[width=\textwidth]{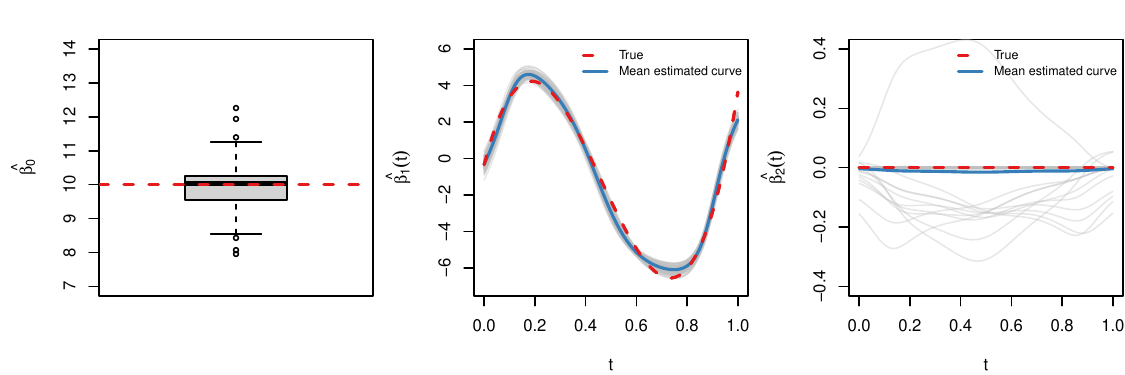}
        \caption{$\sigma^2 = 0.5$}
    \end{subfigure}

    \caption[Simulation Study 1. Estimated functional coefficients per dataset and boxplot of the intercept when $n = 100$.]{Simulation Study 1. Mean estimated curves for the two functional coefficients (blue), individual estimates per simulated dataset (grey), and boxplots of the estimated intercept across 100 simulated datasets, for sample size $n = 100$ and varying error variance ($\sigma^2 = 0.1, 0.5$). True values for the partial functional coefficients and intercept are shown in red.}
    \label{fig:sim1_all_n100_sofr}
\end{figure}

\begin{figure}[ht]
    \centering
    \begin{subfigure}[b]{0.48\textwidth}
        \centering
        \includegraphics[width=\textwidth, page = 1]{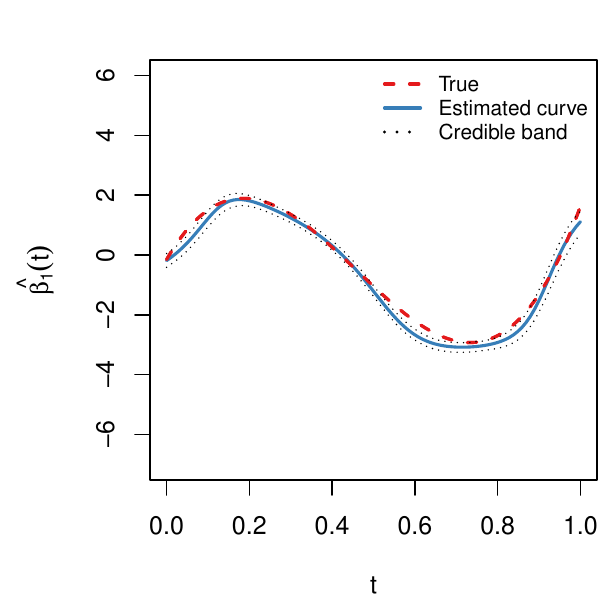}
        \caption{$\sigma^2 = 0.1$}
    \end{subfigure}
    \hfill
    \begin{subfigure}[b]{0.48\textwidth}
        \centering
        \includegraphics[width=\textwidth, page = 1]{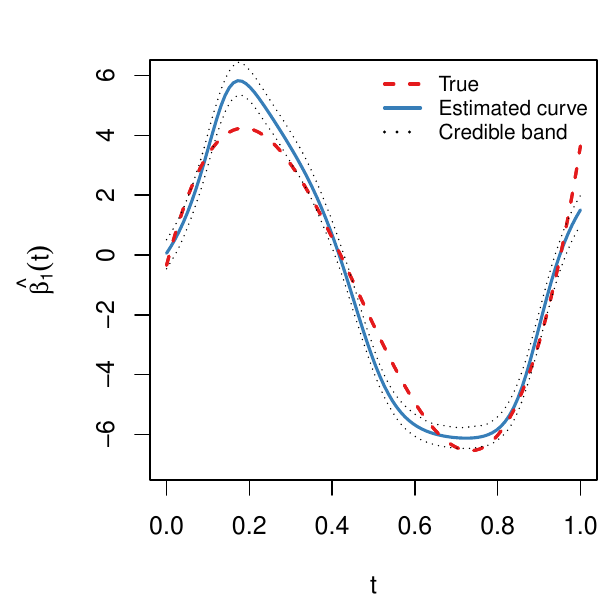}
        \caption{$\sigma^2 = 0.5$}
    \end{subfigure}

    \caption[Simulation Study 1. Estimated non-zero partial functional coefficients with credible bands when $n = 50$.]{Simulation Study 1. Estimated curves for the non-zero partial functional coefficient (blue) with 95\% credible bands (black) for one of the simulated datasets under the scenario with sample size $n = 50$ and error variances $\sigma^2 = 0.1, 0.5$. The true values for the partial functional coefficients are shown in red.}
    \label{fig:sim1_cred_n50_sofr}
\end{figure}

\begin{figure}[ht]
    \centering
    \begin{subfigure}[b]{0.48\textwidth}
        \centering
        \includegraphics[width=\textwidth, page = 1]{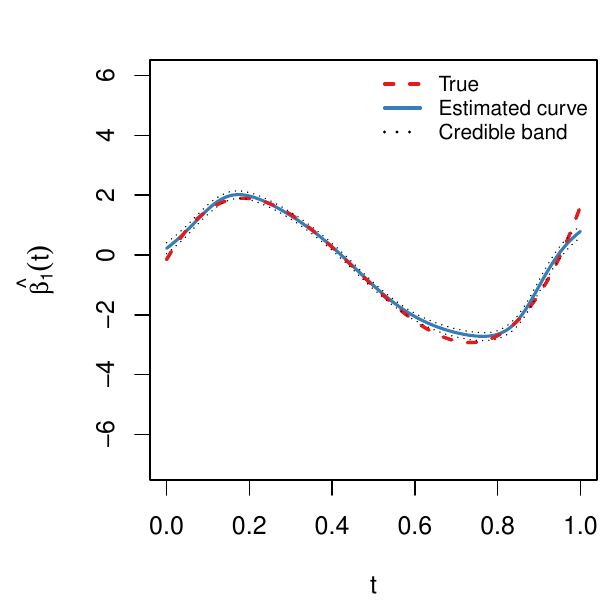}
        \caption{$\sigma^2 = 0.1$}
    \end{subfigure}
    \hfill
    \begin{subfigure}[b]{0.48\textwidth}
        \centering
        \includegraphics[width=\textwidth, page = 1]{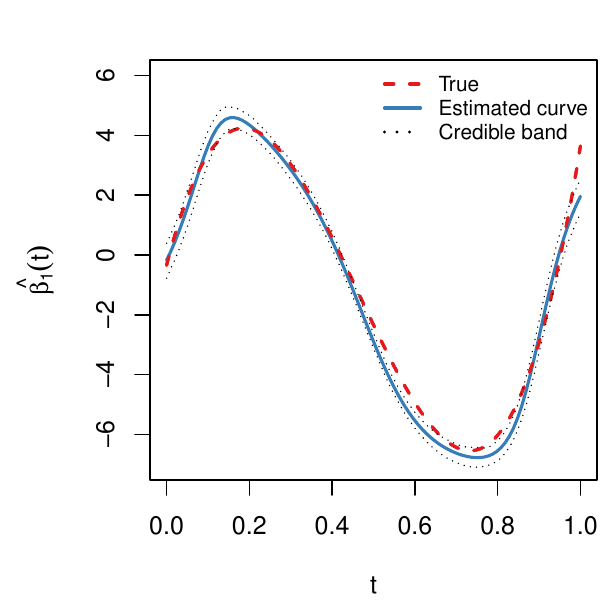}
        \caption{$\sigma^2 = 0.5$}
    \end{subfigure}

    \caption[Simulation Study 1. Estimated non-zero partial functional coefficients with credible bands when $n = 100$.]{Simulation Study 1. Estimated curves for the non-zero partial functional coefficient (blue) with 95\% credible bands (black) for one of the simulated datasets under the scenario with sample size $n = 100$ and error variances $\sigma^2 = 0.1, 0.5$. The true values for the partial functional coefficients are shown in red.}
    \label{fig:sim1_cred_n100_sofr}
\end{figure}

\begin{figure}[ht]
    \centering
    \begin{subfigure}[b]{\textwidth}
        \centering
        \includegraphics[width=.49\textwidth, page=1]{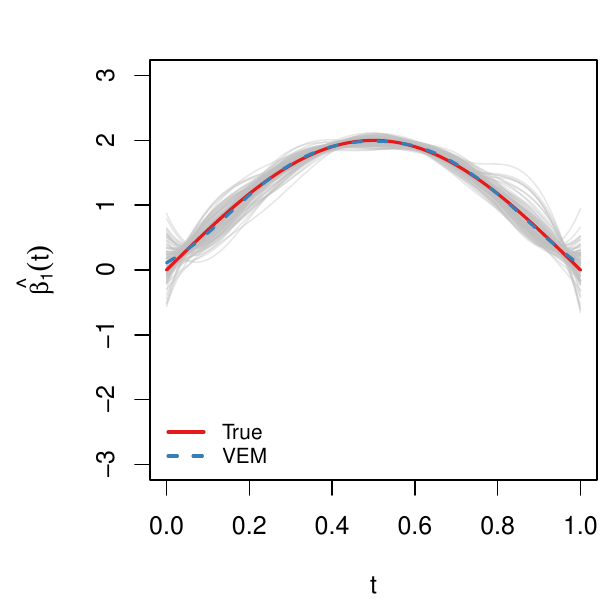}
        \includegraphics[width=.49\textwidth, page=3]{sim2_vem_n100_sigma20.01.pdf}
        \caption{$\sigma^2 = 0.01$}
    \end{subfigure}
    \hfill
    \begin{subfigure}[b]{\textwidth}
        \centering
        \includegraphics[width=.49\textwidth, page=1]{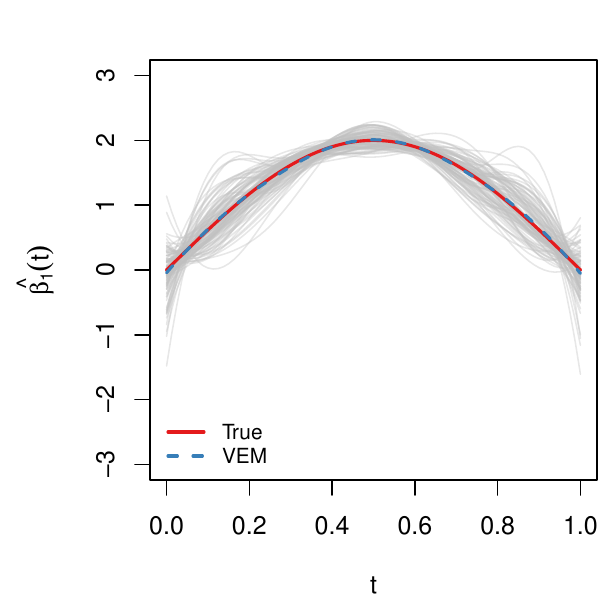}
        \includegraphics[width=.49\textwidth, page=3]{sim2_vem_n100_sigma20.05.pdf}
        \caption{$\sigma^2 = 0.05$}
    \end{subfigure}

    \caption[Simulation Study 2. Estimated curves for the non-zero functional coefficients per dataset for VEM when $n = 100$.]{Simulation Study 2. Mean estimated curves for the non-zero partial functional coefficients obtained from our method (blue) for sample size $n = 100$ and varying error variance ($\sigma^2 = 0.01$ for the plots on the top and $\sigma^2 = 0.05$ for the plots on the bottom). The true values of the non-zero partial functional coefficients are shown in red and individual estimates curves across the 100 simulated datasets obtained from our method are provided in grey.}
    \label{fig:sim2_all_n_100_sofr}
\end{figure}

\begin{figure}[ht]
\centering
\begin{subfigure}[b]{0.48\textwidth}
    \centering
    \includegraphics[width=\textwidth, page = 1]{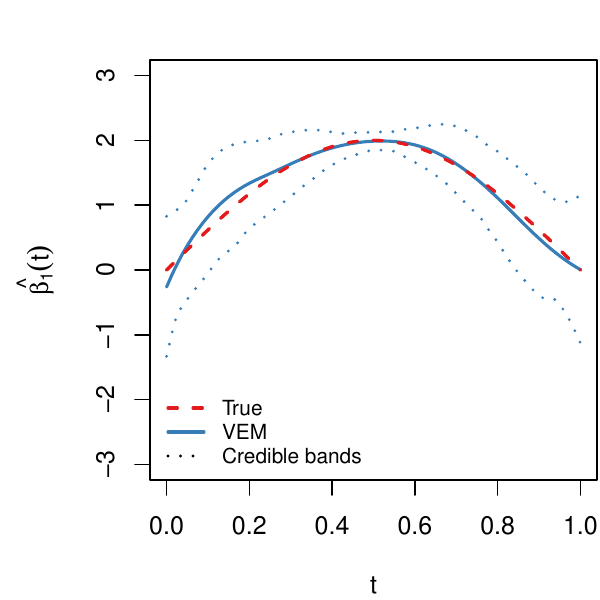}
    \includegraphics[width=\textwidth, page = 3]{sim2_vem_data97_n100_sigma20.01_cred.pdf}
    \caption{$\sigma^2 = 0.01$}
\end{subfigure}
\hfill
\begin{subfigure}[b]{0.48\textwidth}
    \centering
    \includegraphics[width=\textwidth, page = 1]{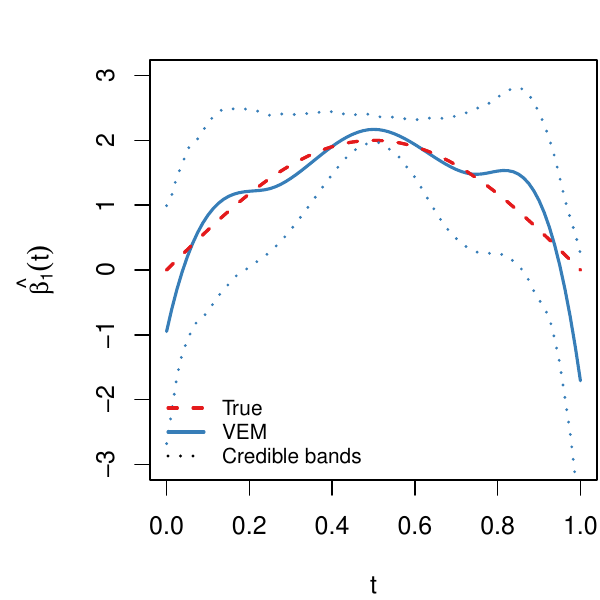}
    \includegraphics[width=\textwidth, page = 3]{sim2_vem_data97_n100_sigma20.05_cred.pdf}
    \caption{$\sigma^2 = 0.05$}
\end{subfigure}

\caption[Simulation Study 2. Estimated curves for non-zero partial functional coefficients with credible bands for VEM when $n = 100$.]{Simulation Study 2. Estimated curves for the non-zero partial functional coefficients from our VEM algorithm (blue) for one of the simulated datasets under the scenario with sample size $n = 100$ and error variances ($\sigma^2 = 0.01$ for plots on the left, and  $\sigma^2 = 0.05$ for plots on the right). A 95\% credible band (dotted curves) was obtained for our method. The true partial functional coefficients are shown in red.}
\label{fig:sim2_cred_n100_sofr}
\end{figure}

\begin{figure}[ht]
    \centering
    \begin{subfigure}[b]{\textwidth}
        \centering
        \includegraphics[width=.49\textwidth, page=1]{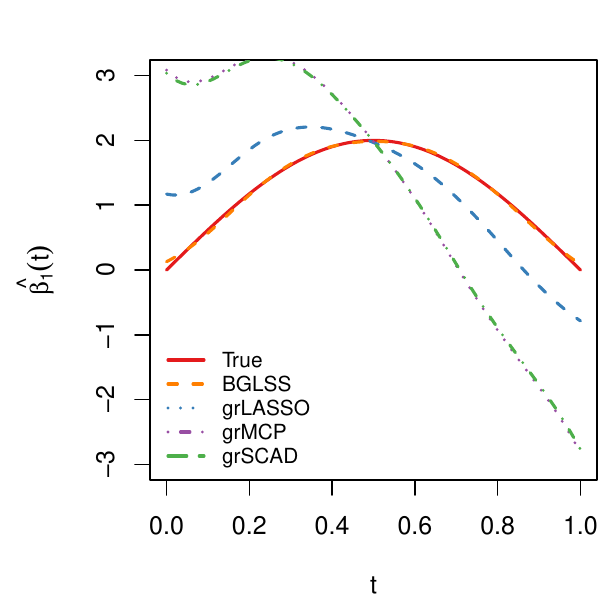}
        \includegraphics[width=.49\textwidth, page=3]{sim2_vem_n100_sigma20.01extra.pdf}
        \caption{$\sigma^2 = 0.01$}
    \end{subfigure}
    \hfill
    \begin{subfigure}[b]{\textwidth}
        \centering
        \includegraphics[width=.49\textwidth, page=1]{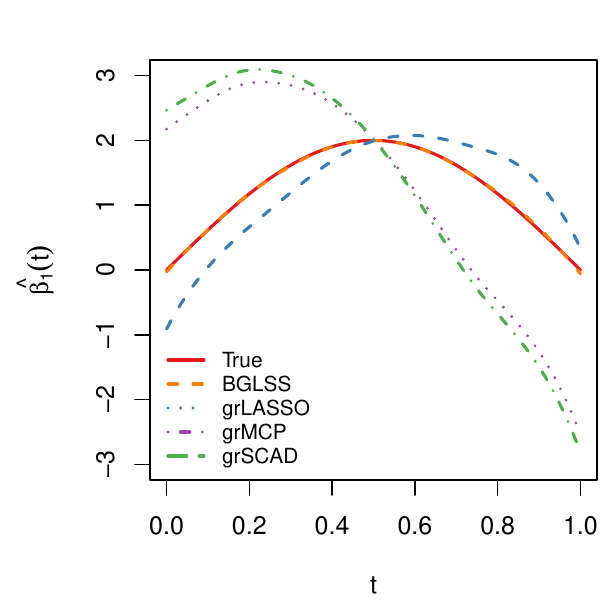}
        \includegraphics[width=.49\textwidth, page=3]{sim2_vem_n100_sigma20.05extra.pdf}
        \caption{$\sigma^2 = 0.05$}
    \end{subfigure}

    \caption{Simulation Study 2. Mean estimated curves for the non-zero partial functional coefficients from BGLSS (orange), gLASSO (blue), gMCP (purple), and gSCAD (green) for sample size $n = 100$ and varying error variance ($\sigma^2 = 0.01$ for the plots on top and $\sigma^2 = 0.05$ for the plots on the bottom). The true values of the partial functional coefficients are shown in red.}
    \label{fig:sim2_all_n_100_sofr_extra}
\end{figure}

\begin{figure}[ht]
    \centering
    \begin{subfigure}[b]{\textwidth}
        \centering
        \includegraphics[width=.49\textwidth, page=1]{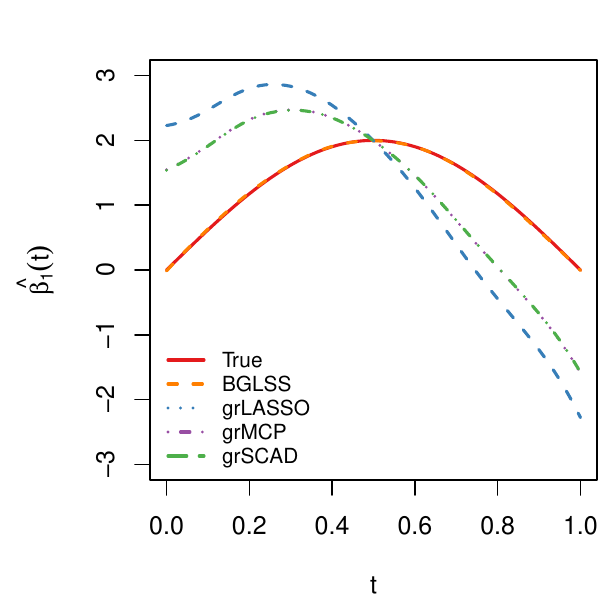}
        \includegraphics[width=.49\textwidth, page=3]{sim2_vem_n400_sigma20.01extra.pdf}
        \caption{$\sigma^2 = 0.01$}
    \end{subfigure}
    \hfill
    \begin{subfigure}[b]{\textwidth}
        \centering
        \includegraphics[width=.49\textwidth, page=1]{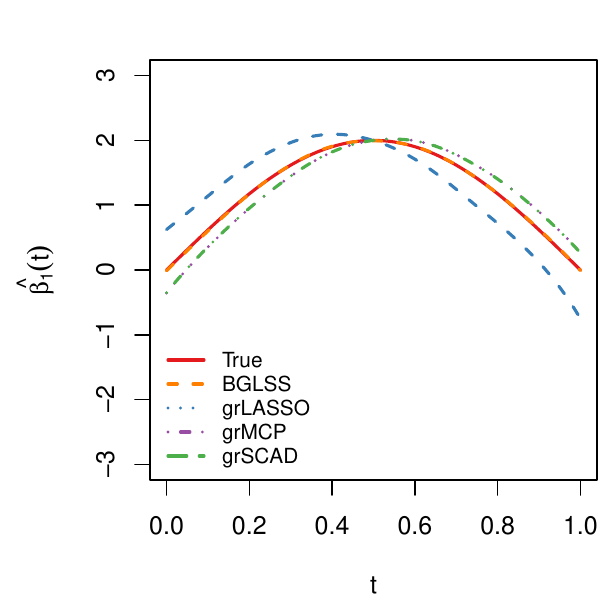}
        \includegraphics[width=.49\textwidth, page=3]{sim2_vem_n400_sigma20.05extra.pdf}
        \caption{$\sigma^2 = 0.05$}
    \end{subfigure}

    \caption{Simulation Study 2. Mean estimated curves for the non-zero partial functional coefficients from BGLSS (orange), gLASSO (blue), gMCP (purple), and gSCAD (green) for sample size $n = 400$ and varying error variance ($\sigma^2 = 0.01$ for the plots on the top and $\sigma^2 = 0.05$ for the plots on the bottom). The true values of the partial functional coefficients are shown in red.}
    \label{fig:sim2_all_n_400_sofr_extra}
\end{figure}

\begin{figure}[ht]
    \centering
    \begin{subfigure}[b]{.38\textwidth}
        \centering
        \includegraphics[width=\textwidth, page=1]{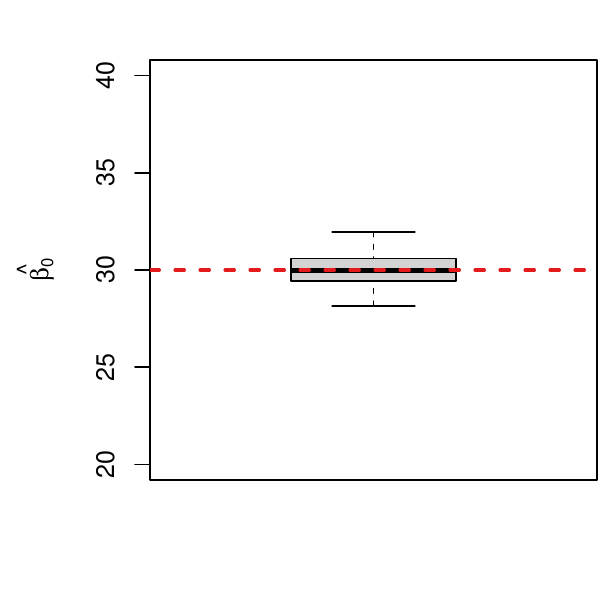}
        \includegraphics[width=\textwidth, page=2]{sim3_vem_n50_sigma20.1.pdf}
        \caption{$\sigma^2 = 0.1$}
    \end{subfigure}
%    \hfill
    \begin{subfigure}[b]{.38\textwidth}
        \centering
        \includegraphics[width=\textwidth, page=1]{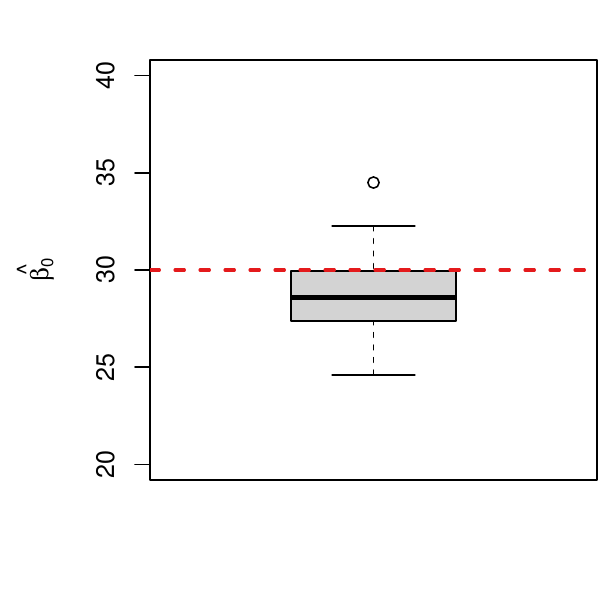}
        \includegraphics[width=\textwidth, page=2]{sim3_vem_n50_sigma20.5.pdf}
        \caption{$\sigma^2 = 0.5$}
    \end{subfigure}
    \caption[Simulation Study 3. Estimated non-zero partial functional coefficients per dataset and boxplot of the intercept when $n = 50$.]{Simulation Study 3. Mean estimated curves (blue) for the non-zero partial functional coefficients, individual estimated curves for each simulated dataset (grey) and boxplot of the estimated intercept across 100 simulated datasets, for sample size $n = 50$ and varying error variance ($\sigma^2 = 0.1$ for the tops on the left and  $\sigma^2 = 0.5$ for the plots on the right). The true values of the non-zero partial functional coefficient and intercept are shown in red.}
   \label{fig:sim3_all_n50_sofr}
\end{figure}

\begin{figure}[ht]
    \centering

     \begin{subfigure}[b]{0.48\textwidth}
        \centering
        \includegraphics[width=\textwidth, page = 1]{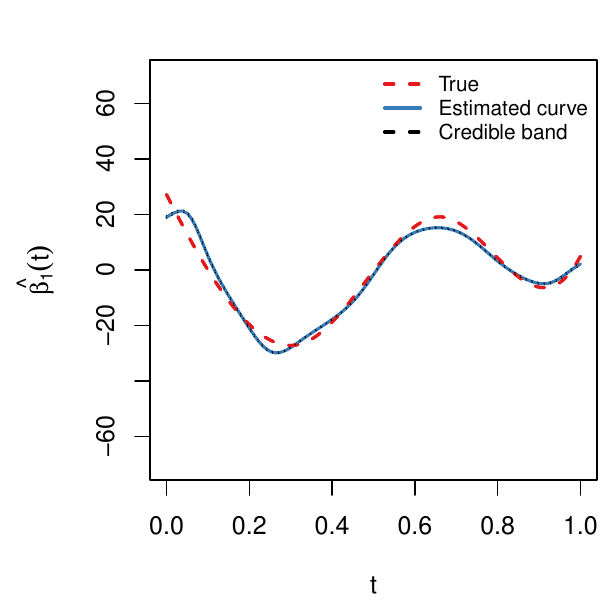}
        \caption{$\sigma^2 = 0.1$}
    \end{subfigure}
    \hfill
    \begin{subfigure}[b]{0.48\textwidth}
        \centering
        \includegraphics[width=\textwidth, page = 1]{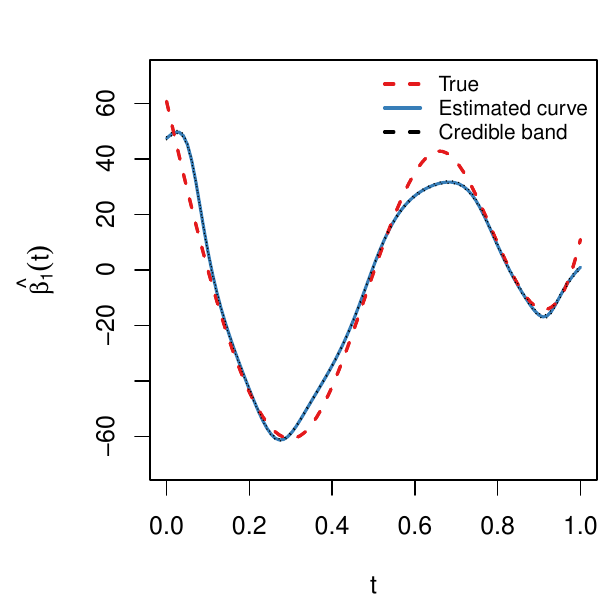}
        \caption{$\sigma^2 = 0.5$}
    \end{subfigure}

    \caption[Simulation Study 3. Estimated non-zero partial functional coefficients with credible bands when $n = 50$.]{Simulation Study 3. Estimated curves (blue) for the non-zero partial functional coefficients with corresponding 95\% credible bands for one of the simulated datasets under the scenario with sample size $n = 50$ and error variances $\sigma^2 = 0.1, 0.5$. The true non-zero partial functional coefficients are shown in red.}
    \label{fig:sim3_n50cred_sofr}
\end{figure}

\begin{figure}[ht]
    \centering
     \begin{subfigure}[b]{0.48\textwidth}
        \centering
        \includegraphics[width=\textwidth, page = 1]{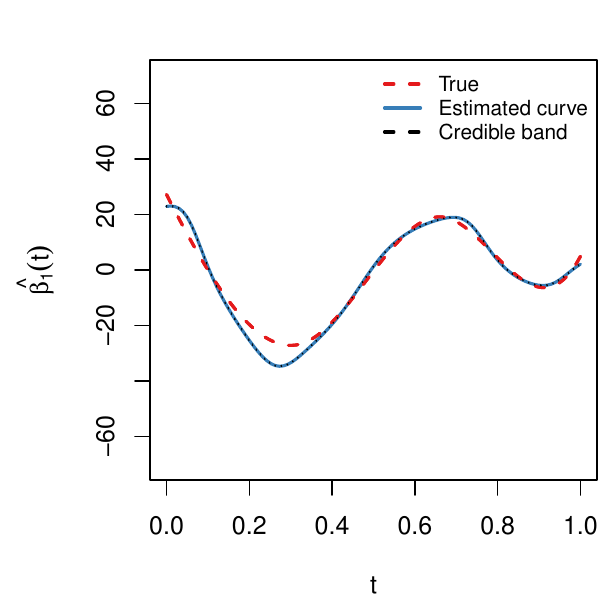}
        \caption{$\sigma^2 = 0.1$}
    \end{subfigure}
    \hfill
    \begin{subfigure}[b]{0.48\textwidth}
        \centering
        \includegraphics[width=\textwidth, page = 1]{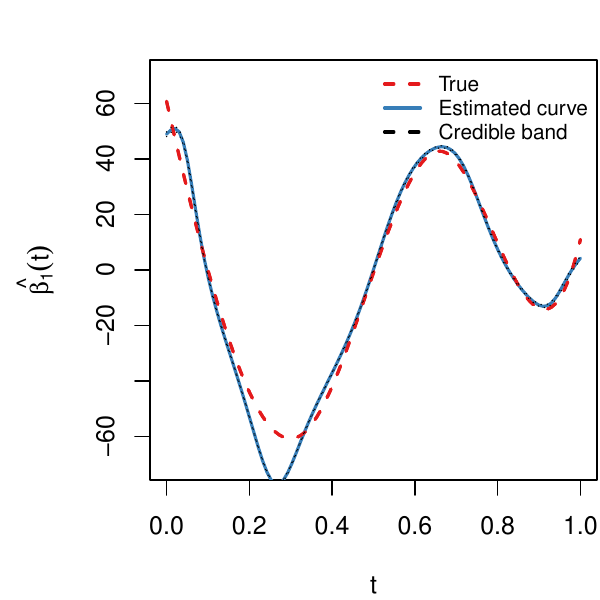}
        \caption{$\sigma^2 = 0.5$}
    \end{subfigure}
    \caption[Simulation Study 3. Estimated non-zero partial functional coefficient with credible bands when $n = 100$.]{Simulation Study 3. Estimated curves (blue) for the non-zero partial functional coefficient with corresponding 95\% credible bands for one of the simulated datasets under the scenario with sample size $n = 100$ and error variances $\sigma^2 = 0.1, 0.5$. The true partial non-zero functional coefficients is shown in red.}
    \label{fig:sim3_cred_n_100_sofr}
\end{figure}
\clearpage

\section{Additional figures for real data applications}
\label{ap:res_data}

In this section, we include the estimated partial functional coefficients obtained from the alternative methods compared in the analyses of sugar spectra and Japan weather datasets.

\begin{figure}[ht]
    \centering
    \begin{subfigure}[b]{0.27\textwidth}
        \centering
        \includegraphics[width=\textwidth, page = 1]{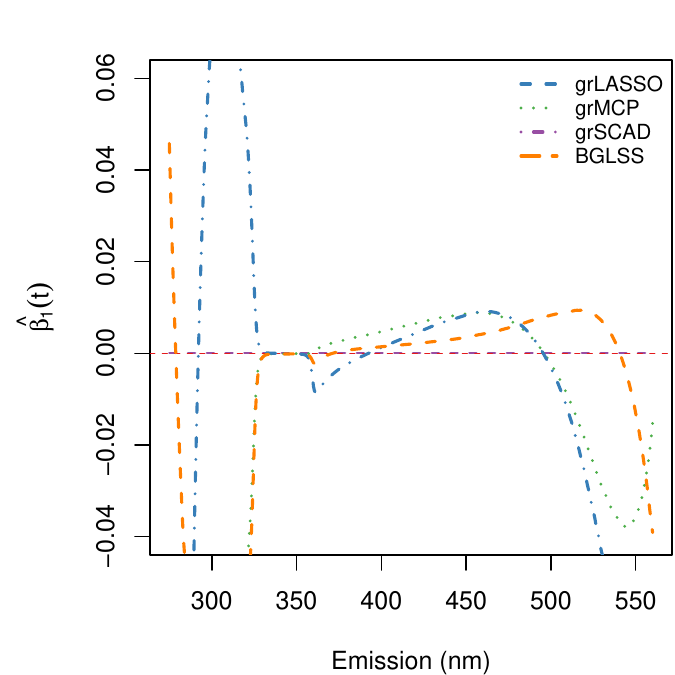}
        \caption{Excitation 230 nm}
    \end{subfigure}
    \begin{subfigure}[b]{0.27\textwidth}
        \centering
        \includegraphics[width=\textwidth, page = 2]{Comparative_results_sugar_vem.pdf}
        \caption{Excitation 240 nm}
    \end{subfigure}
    \begin{subfigure}[b]{0.27\textwidth}
        \centering
        \includegraphics[width=\textwidth, page = 3]{Comparative_results_sugar_vem.pdf}
        \caption{Excitation 255 nm}
    \end{subfigure}
     \begin{subfigure}[b]{0.27\textwidth}
        \centering
        \includegraphics[width=\textwidth, page = 4]{Comparative_results_sugar_vem.pdf}
        \caption{Excitation 290 nm}
    \end{subfigure}
     \begin{subfigure}[b]{0.27\textwidth}
        \centering
        \includegraphics[width=\textwidth, page = 5]{Comparative_results_sugar_vem.pdf}
        \caption{Excitation 305 nm}
    \end{subfigure}
     \begin{subfigure}[b]{0.27\textwidth}
        \centering
        \includegraphics[width=\textwidth, page = 6]{Comparative_results_sugar_vem.pdf}
        \caption{Excitation 325 nm}
    \end{subfigure}
     \begin{subfigure}[b]{0.27\textwidth}
        \centering
        \includegraphics[width=\textwidth, page = 7]{Comparative_results_sugar_vem.pdf}
        \caption{Excitation 340 nm}
    \end{subfigure}

    \caption[Sugar spectra dataset. Estimated functional coefficients for other methods.]{Sugar spectra dataset. The estimated curves for the functional coefficients corresponding to the seven excitation wavelengths, 230, 240, 255, 290, 305, 325, 340 nm, are shown using grLASSO (blue), grMCP (green), grSCAD (purple), and BGLSS (orange). A horizontal red line at zero is included for reference.}
    \label{fig:sugar_betas_alter}
\end{figure}

\begin{figure}[ht]
    \centering
    \begin{subfigure}[b]{0.35\textwidth}
        \centering
        \includegraphics[width=\textwidth, page = 1]{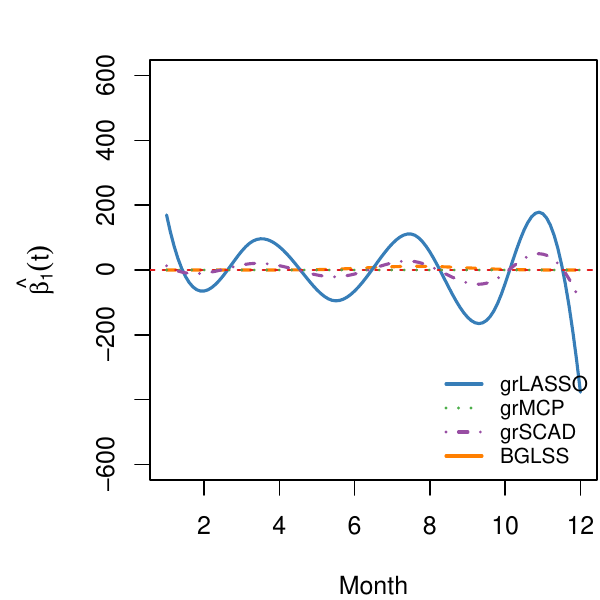}
        \caption{Temperature}
    \end{subfigure}
    \begin{subfigure}[b]{0.35\textwidth}
        \centering
        \includegraphics[width=\textwidth, page = 2]{Comparative_results_jma_vem.pdf}
        \caption{Maximum temperature}
    \end{subfigure}
    \begin{subfigure}[b]{0.35\textwidth}
        \centering
        \includegraphics[width=\textwidth, page = 3]{Comparative_results_jma_vem.pdf}
        \caption{Minimum temperature}
    \end{subfigure}
    \begin{subfigure}[b]{0.35\textwidth}
        \centering
        \includegraphics[width=\textwidth, page = 4]{Comparative_results_jma_vem.pdf}
        \caption{Pressure}
    \end{subfigure}
    \begin{subfigure}[b]{0.35\textwidth}
        \centering
        \includegraphics[width=\textwidth, page = 5]{Comparative_results_jma_vem.pdf}
        \caption{Humidity}
    \end{subfigure}
    \begin{subfigure}[b]{0.35\textwidth}
        \centering
        \includegraphics[width=\textwidth, page = 6]{Comparative_results_jma_vem.pdf}
        \caption{Daylight duration}
    \end{subfigure}

    \caption[Japan weather data. Estimated functional coefficients for other methods.]{Japan weather dataset. Estimated curves for the functional coefficients associated to the weather information for grLASSO (blue), grMCP (green), grSCAD (purple), and BGLSS (orange). A horizontal red line at zero is included for reference.}
    \label{fig:jma_betas_other}
\end{figure}

\clearpage
\end{document}
