# Supplementary material for: Variational Inference for Variable Selection in Scalar-on-Function Regression
Source: arXiv:2603.07856 source file (2026-03-09)
Supplement: Supplementary file 4 [file supp_sofr_sim.tex]

\section{Additional figures for simulation studies}
\label{ap:res_sim}
\setcounter{figure}{0}

In this section, we include additional figures from the simulations studies described in the main text.

\begin{figure}[ht]
    \centering
    \begin{subfigure}[b]{\textwidth}
        \centering
        \includegraphics[width=\textwidth]{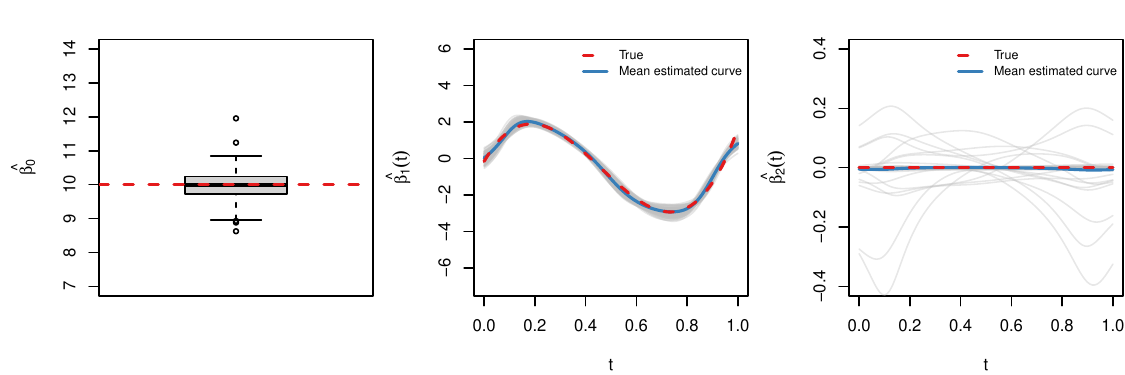}
        \caption{$\sigma^2 = 0.1$}
    \end{subfigure}
    \hfill
    \begin{subfigure}[b]{\textwidth}
        \centering
        \includegraphics[width=\textwidth]{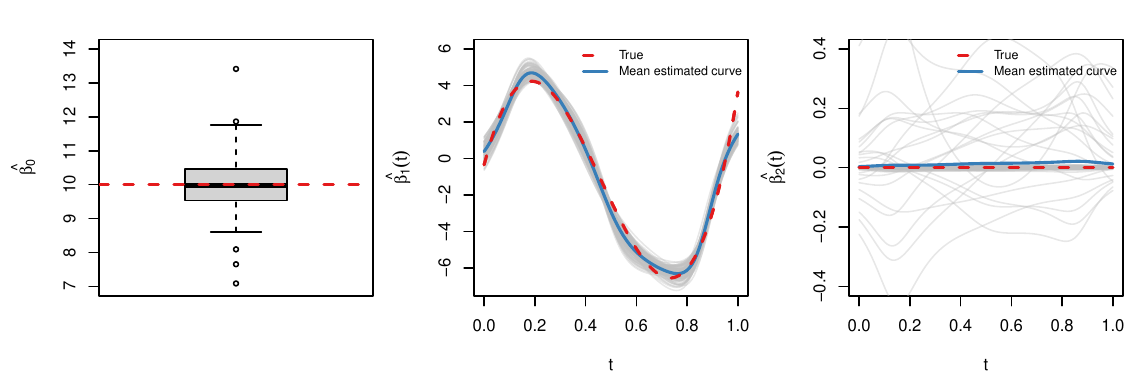}
        \caption{$\sigma^2 = 0.5$}
    \end{subfigure}

    \caption[Simulation Study 1. Estimated functional coefficients per dataset and boxplot of the intercept when $n = 50$.]{Simulation Study 1. Mean estimated curves for the two functional coefficients (blue), individual estimates per simulated dataset (grey), and boxplots of the estimated intercept across 100 simulated datasets, for sample size $n = 50$ and varying error variance ($\sigma^2 = 0.1, 0.5$). True values for the partial functional coefficients and intercept are shown in red.}
    \label{fig:sim1_all_n50_sofr}
\end{figure}

\begin{figure}[ht]
    \centering
    \begin{subfigure}[b]{\textwidth}
        \centering
        \includegraphics[width=\textwidth]{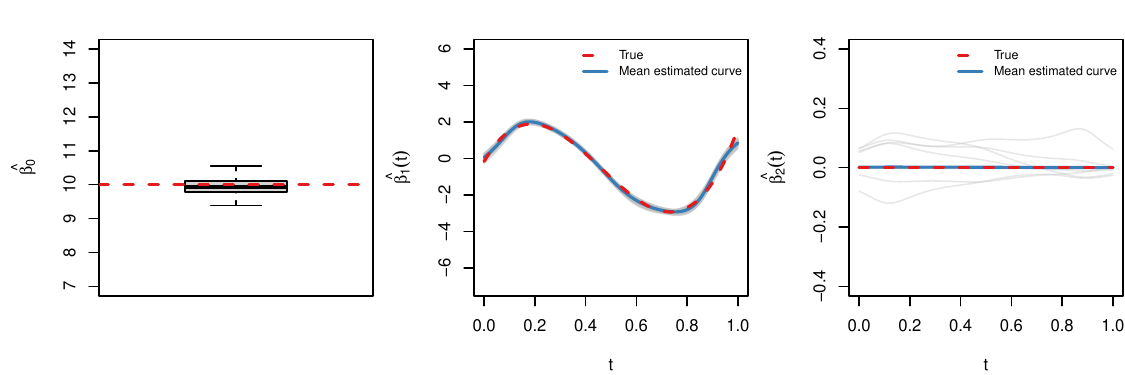}
        \caption{$\sigma^2 = 0.1$}
    \end{subfigure}
    \begin{subfigure}[b]{\textwidth}
        \centering
        \includegraphics[width=\textwidth]{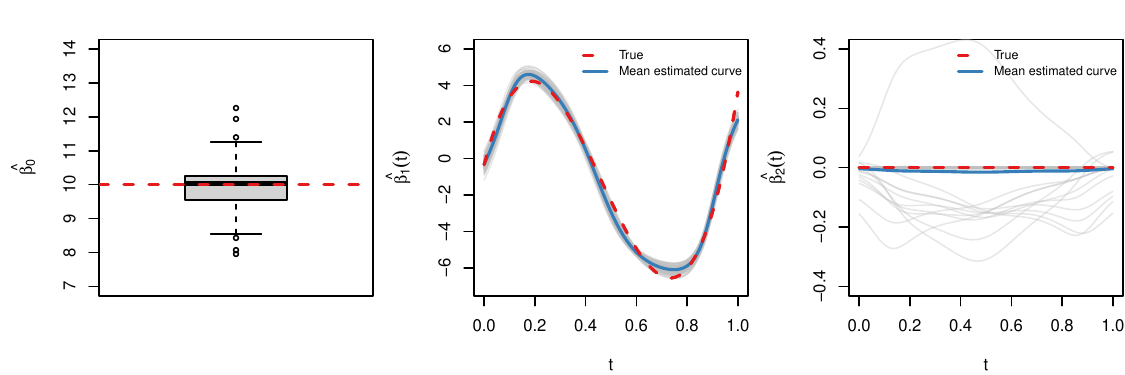}
        \caption{$\sigma^2 = 0.5$}
    \end{subfigure}

    \caption[Simulation Study 1. Estimated functional coefficients per dataset and boxplot of the intercept when $n = 100$.]{Simulation Study 1. Mean estimated curves for the two functional coefficients (blue), individual estimates per simulated dataset (grey), and boxplots of the estimated intercept across 100 simulated datasets, for sample size $n = 100$ and varying error variance ($\sigma^2 = 0.1, 0.5$). True values for the partial functional coefficients and intercept are shown in red.}
    \label{fig:sim1_all_n100_sofr}
\end{figure}

\begin{figure}[ht]
    \centering
    \begin{subfigure}[b]{0.48\textwidth}
        \centering
        \includegraphics[width=\textwidth, page = 1]{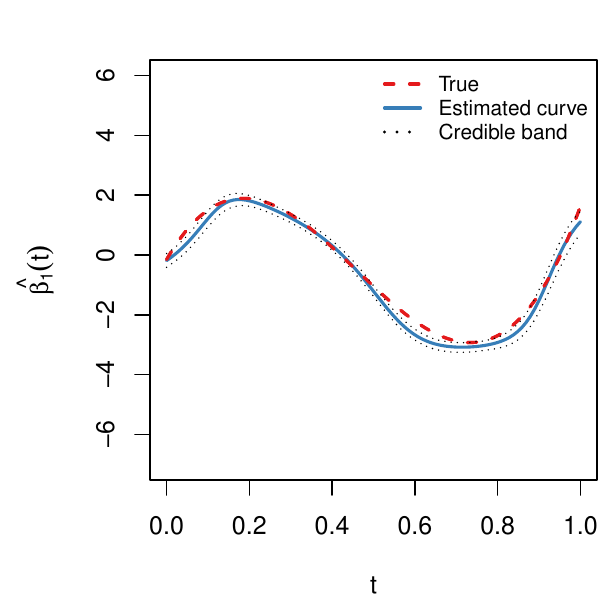}
        \caption{$\sigma^2 = 0.1$}
    \end{subfigure}
    \hfill
    \begin{subfigure}[b]{0.48\textwidth}
        \centering
        \includegraphics[width=\textwidth, page = 1]{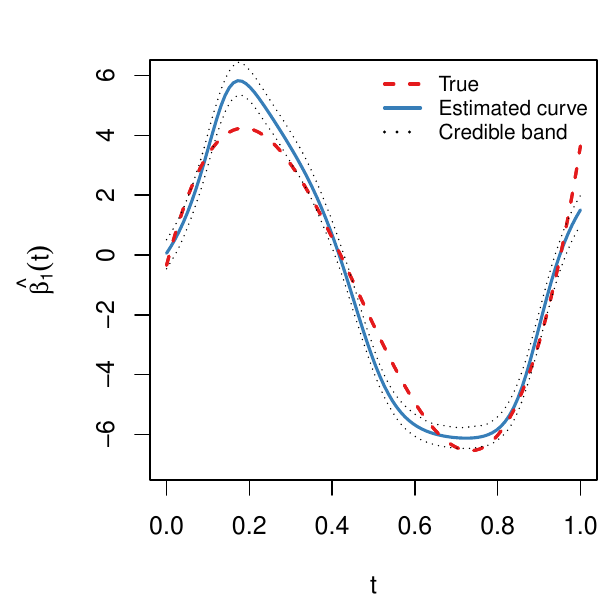}
        \caption{$\sigma^2 = 0.5$}
    \end{subfigure}

    \caption[Simulation Study 1. Estimated non-zero partial functional coefficients with credible bands when $n = 50$.]{Simulation Study 1. Estimated curves for the non-zero partial functional coefficient (blue) with 95\% credible bands (black) for one of the simulated datasets under the scenario with sample size $n = 50$ and error variances $\sigma^2 = 0.1, 0.5$. The true values for the partial functional coefficients are shown in red.}
    \label{fig:sim1_cred_n50_sofr}
\end{figure}

\begin{figure}[ht]
    \centering
    \begin{subfigure}[b]{0.48\textwidth}
        \centering
        \includegraphics[width=\textwidth, page = 1]{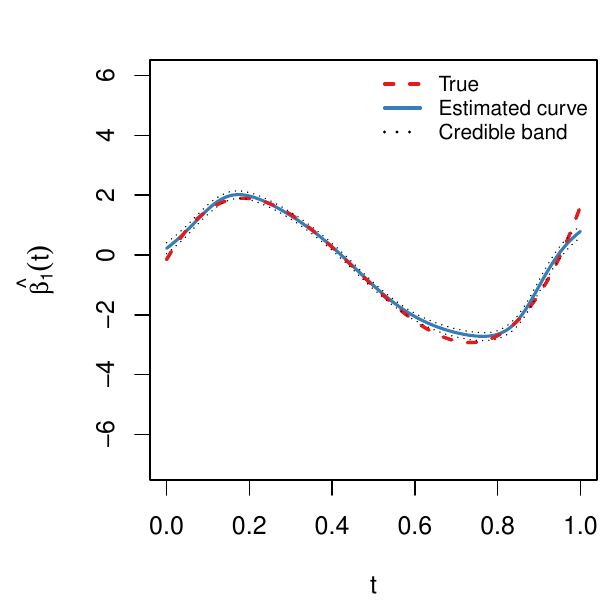}
        \caption{$\sigma^2 = 0.1$}
    \end{subfigure}
    \hfill
    \begin{subfigure}[b]{0.48\textwidth}
        \centering
        \includegraphics[width=\textwidth, page = 1]{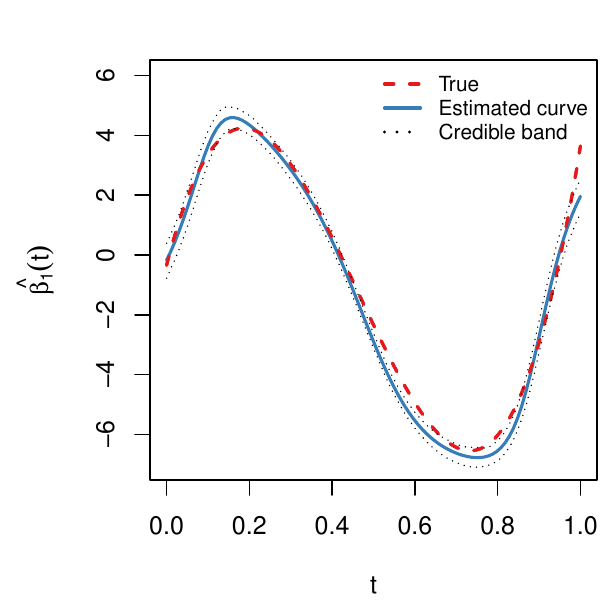}
        \caption{$\sigma^2 = 0.5$}
    \end{subfigure}

    \caption[Simulation Study 1. Estimated non-zero partial functional coefficients with credible bands when $n = 100$.]{Simulation Study 1. Estimated curves for the non-zero partial functional coefficient (blue) with 95\% credible bands (black) for one of the simulated datasets under the scenario with sample size $n = 100$ and error variances $\sigma^2 = 0.1, 0.5$. The true values for the partial functional coefficients are shown in red.}
    \label{fig:sim1_cred_n100_sofr}
\end{figure}

\begin{figure}[ht]
    \centering
    \begin{subfigure}[b]{\textwidth}
        \centering
        \includegraphics[width=.49\textwidth, page=1]{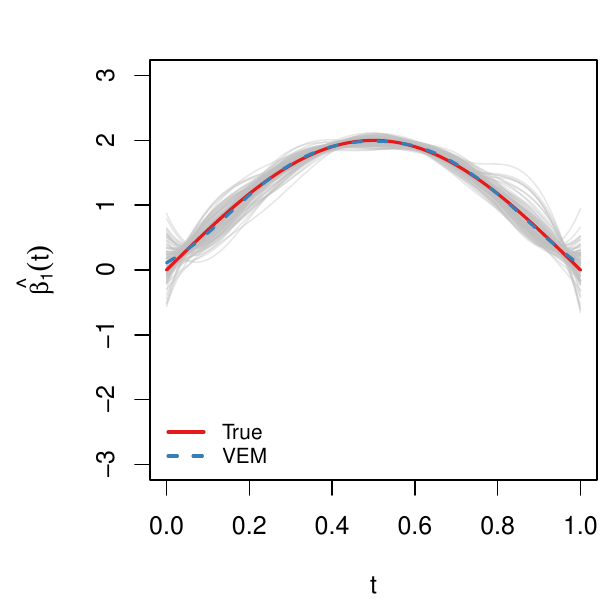}
        \includegraphics[width=.49\textwidth, page=3]{sim2_vem_n100_sigma20.01.pdf}
        \caption{$\sigma^2 = 0.01$}
    \end{subfigure}
    \hfill
    \begin{subfigure}[b]{\textwidth}
        \centering
        \includegraphics[width=.49\textwidth, page=1]{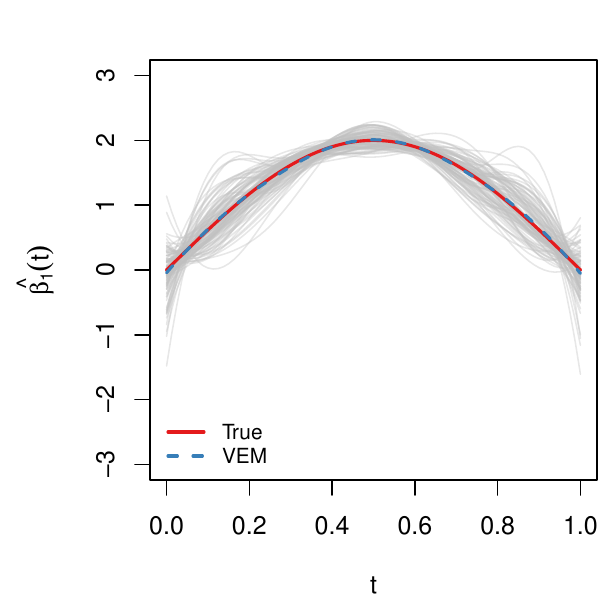}
        \includegraphics[width=.49\textwidth, page=3]{sim2_vem_n100_sigma20.05.pdf}
        \caption{$\sigma^2 = 0.05$}
    \end{subfigure}

    \caption[Simulation Study 2. Estimated curves for the non-zero functional coefficients per dataset for VEM when $n = 100$.]{Simulation Study 2. Mean estimated curves for the non-zero partial functional coefficients obtained from our method (blue) for sample size $n = 100$ and varying error variance ($\sigma^2 = 0.01$ for the plots on the top and $\sigma^2 = 0.05$ for the plots on the bottom). The true values of the non-zero partial functional coefficients are shown in red and individual estimates curves across the 100 simulated datasets obtained from our method are provided in grey.}
    \label{fig:sim2_all_n_100_sofr}
\end{figure}

\begin{figure}[ht]
\centering
\begin{subfigure}[b]{0.48\textwidth}
    \centering
    \includegraphics[width=\textwidth, page = 1]{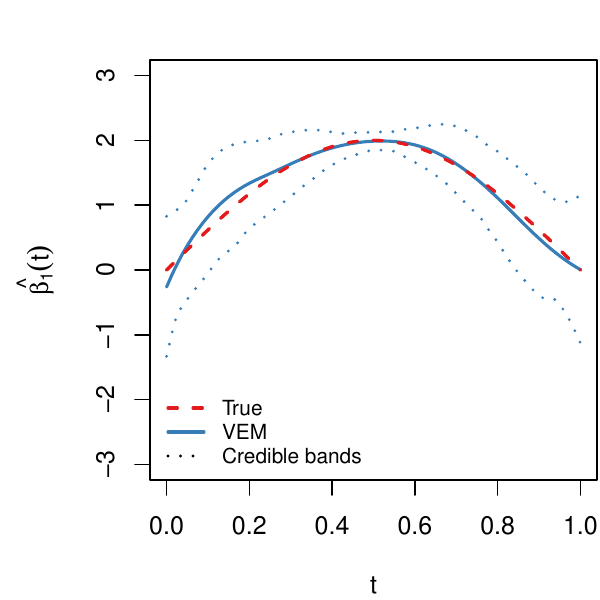}
    \includegraphics[width=\textwidth, page = 3]{sim2_vem_data97_n100_sigma20.01_cred.pdf}
    \caption{$\sigma^2 = 0.01$}
\end{subfigure}
\hfill
\begin{subfigure}[b]{0.48\textwidth}
    \centering
    \includegraphics[width=\textwidth, page = 1]{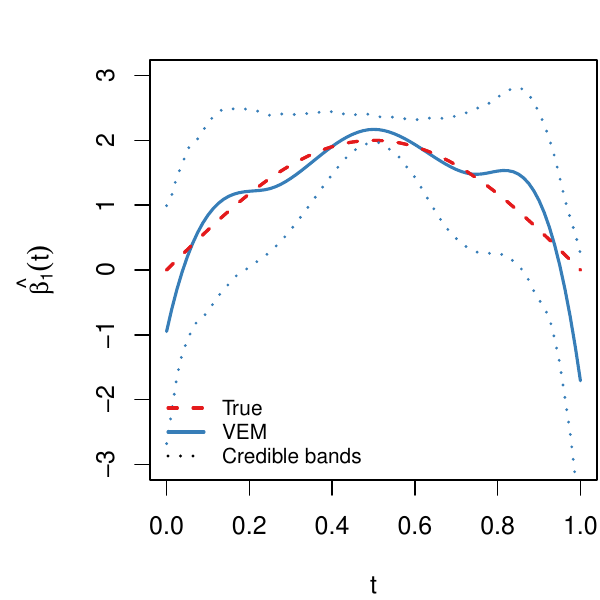}
    \includegraphics[width=\textwidth, page = 3]{sim2_vem_data97_n100_sigma20.05_cred.pdf}
    \caption{$\sigma^2 = 0.05$}
\end{subfigure}

\caption[Simulation Study 2. Estimated curves for non-zero partial functional coefficients with credible bands for VEM when $n = 100$.]{Simulation Study 2. Estimated curves for the non-zero partial functional coefficients from our VEM algorithm (blue) for one of the simulated datasets under the scenario with sample size $n = 100$ and error variances ($\sigma^2 = 0.01$ for plots on the left, and  $\sigma^2 = 0.05$ for plots on the right). A 95\% credible band (dotted curves) was obtained for our method. The true partial functional coefficients are shown in red.}
\label{fig:sim2_cred_n100_sofr}
\end{figure}

\begin{figure}[ht]
    \centering
    \begin{subfigure}[b]{\textwidth}
        \centering
        \includegraphics[width=.49\textwidth, page=1]{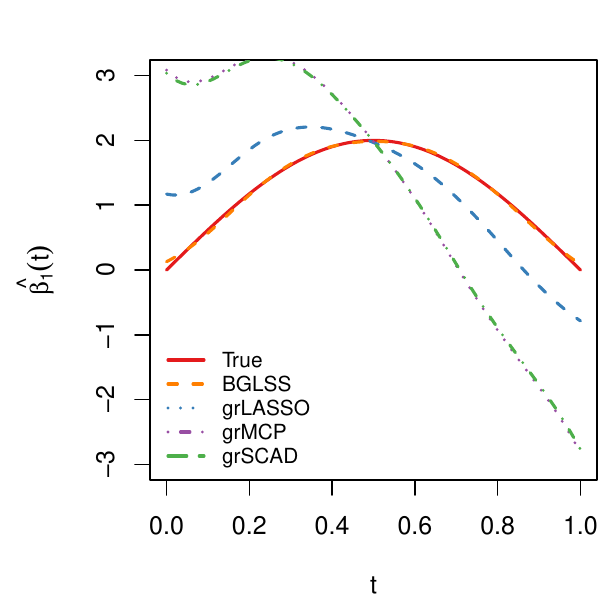}
        \includegraphics[width=.49\textwidth, page=3]{sim2_vem_n100_sigma20.01extra.pdf}
        \caption{$\sigma^2 = 0.01$}
    \end{subfigure}
    \hfill
    \begin{subfigure}[b]{\textwidth}
        \centering
        \includegraphics[width=.49\textwidth, page=1]{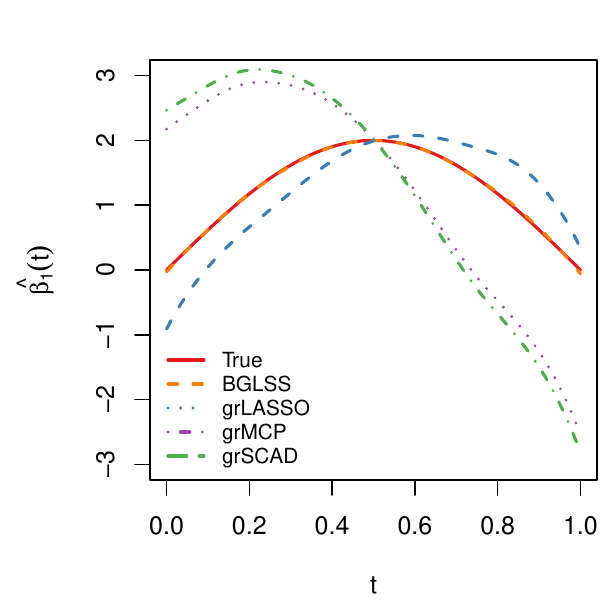}
        \includegraphics[width=.49\textwidth, page=3]{sim2_vem_n100_sigma20.05extra.pdf}
        \caption{$\sigma^2 = 0.05$}
    \end{subfigure}

    \caption{Simulation Study 2. Mean estimated curves for the non-zero partial functional coefficients from BGLSS (orange), gLASSO (blue), gMCP (purple), and gSCAD (green) for sample size $n = 100$ and varying error variance ($\sigma^2 = 0.01$ for the plots on top and $\sigma^2 = 0.05$ for the plots on the bottom). The true values of the partial functional coefficients are shown in red.}
    \label{fig:sim2_all_n_100_sofr_extra}
\end{figure}

\begin{figure}[ht]
    \centering
    \begin{subfigure}[b]{\textwidth}
        \centering
        \includegraphics[width=.49\textwidth, page=1]{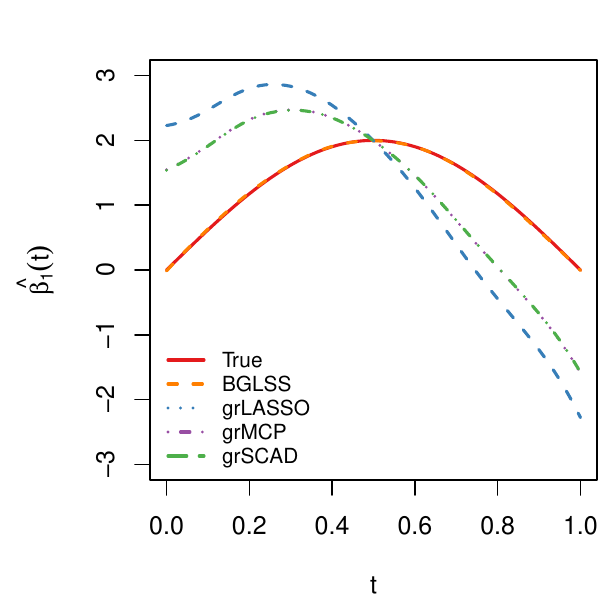}
        \includegraphics[width=.49\textwidth, page=3]{sim2_vem_n400_sigma20.01extra.pdf}
        \caption{$\sigma^2 = 0.01$}
    \end{subfigure}
    \hfill
    \begin{subfigure}[b]{\textwidth}
        \centering
        \includegraphics[width=.49\textwidth, page=1]{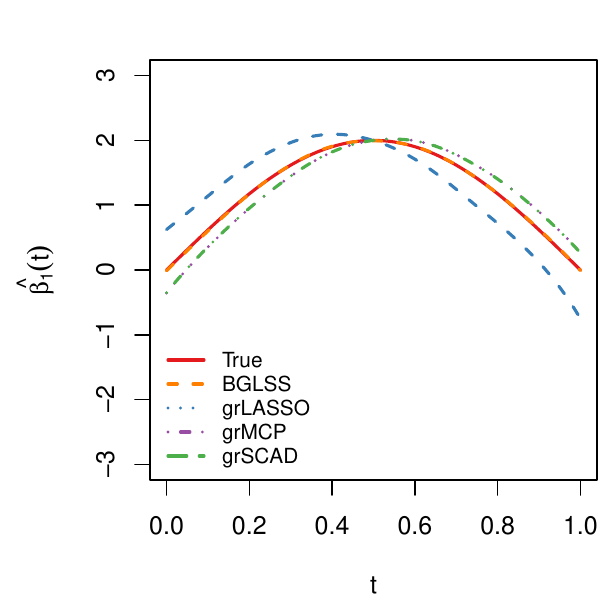}
        \includegraphics[width=.49\textwidth, page=3]{sim2_vem_n400_sigma20.05extra.pdf}
        \caption{$\sigma^2 = 0.05$}
    \end{subfigure}

    \caption{Simulation Study 2. Mean estimated curves for the non-zero partial functional coefficients from BGLSS (orange), gLASSO (blue), gMCP (purple), and gSCAD (green) for sample size $n = 400$ and varying error variance ($\sigma^2 = 0.01$ for the plots on the top and $\sigma^2 = 0.05$ for the plots on the bottom). The true values of the partial functional coefficients are shown in red.}
    \label{fig:sim2_all_n_400_sofr_extra}
\end{figure}

\begin{figure}[ht]
    \centering
    \begin{subfigure}[b]{.38\textwidth}
        \centering
        \includegraphics[width=\textwidth, page=1]{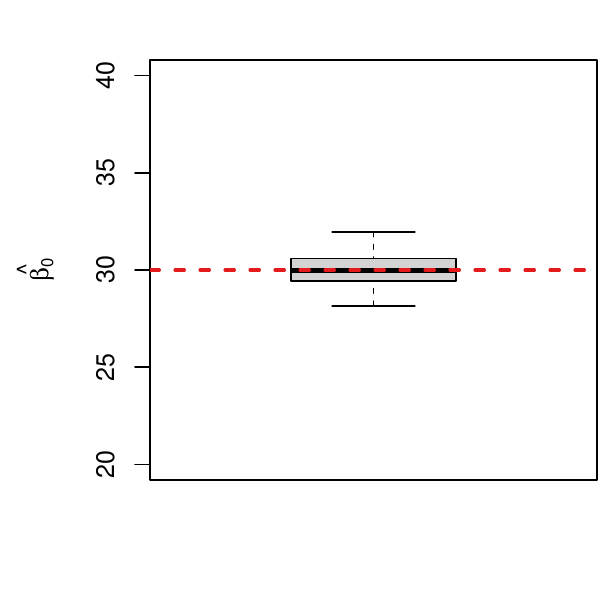}
        \includegraphics[width=\textwidth, page=2]{sim3_vem_n50_sigma20.1.pdf}
        \caption{$\sigma^2 = 0.1$}
    \end{subfigure}
%    \hfill
    \begin{subfigure}[b]{.38\textwidth}
        \centering
        \includegraphics[width=\textwidth, page=1]{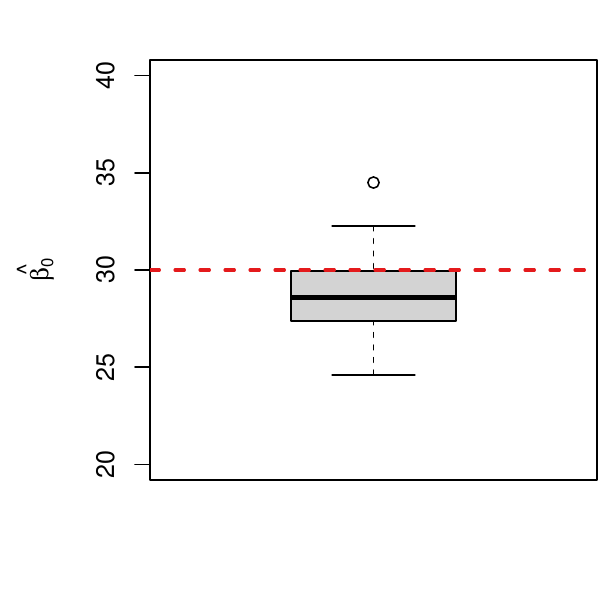}
        \includegraphics[width=\textwidth, page=2]{sim3_vem_n50_sigma20.5.pdf}
        \caption{$\sigma^2 = 0.5$}
    \end{subfigure}
    \caption[Simulation Study 3. Estimated non-zero partial functional coefficients per dataset and boxplot of the intercept when $n = 50$.]{Simulation Study 3. Mean estimated curves (blue) for the non-zero partial functional coefficients, individual estimated curves for each simulated dataset (grey) and boxplot of the estimated intercept across 100 simulated datasets, for sample size $n = 50$ and varying error variance ($\sigma^2 = 0.1$ for the tops on the left and  $\sigma^2 = 0.5$ for the plots on the right). The true values of the non-zero partial functional coefficient and intercept are shown in red.}
   \label{fig:sim3_all_n50_sofr}
\end{figure}

\begin{figure}[ht]
    \centering

     \begin{subfigure}[b]{0.48\textwidth}
        \centering
        \includegraphics[width=\textwidth, page = 1]{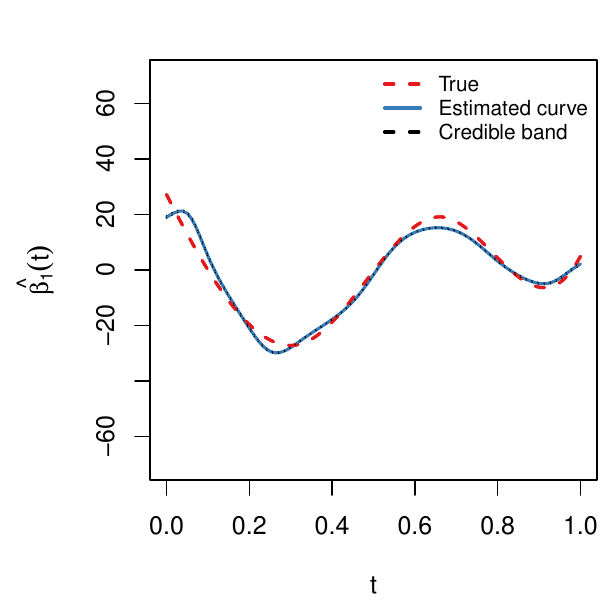}
        \caption{$\sigma^2 = 0.1$}
    \end{subfigure}
    \hfill
    \begin{subfigure}[b]{0.48\textwidth}
        \centering
        \includegraphics[width=\textwidth, page = 1]{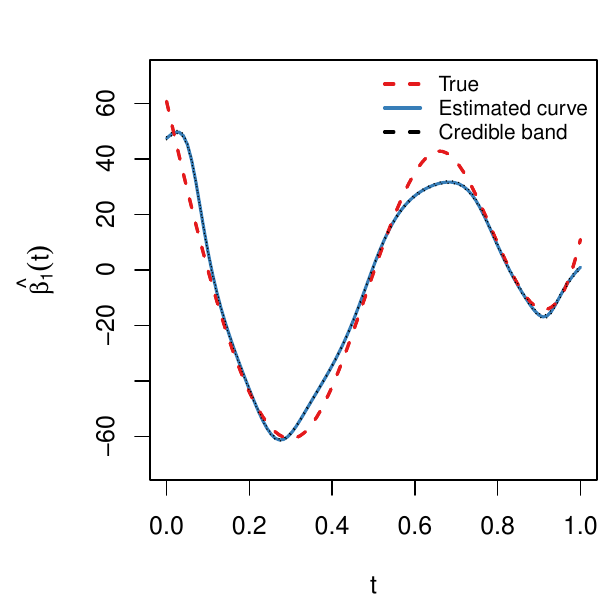}
        \caption{$\sigma^2 = 0.5$}
    \end{subfigure}

    \caption[Simulation Study 3. Estimated non-zero partial functional coefficients with credible bands when $n = 50$.]{Simulation Study 3. Estimated curves (blue) for the non-zero partial functional coefficients with corresponding 95\% credible bands for one of the simulated datasets under the scenario with sample size $n = 50$ and error variances $\sigma^2 = 0.1, 0.5$. The true non-zero partial functional coefficients are shown in red.}
    \label{fig:sim3_n50cred_sofr}
\end{figure}

\begin{figure}[ht]
    \centering
     \begin{subfigure}[b]{0.48\textwidth}
        \centering
        \includegraphics[width=\textwidth, page = 1]{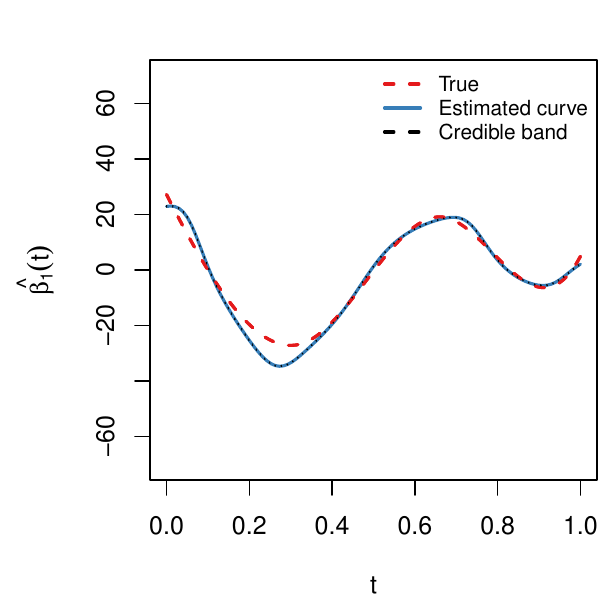}
        \caption{$\sigma^2 = 0.1$}
    \end{subfigure}
    \hfill
    \begin{subfigure}[b]{0.48\textwidth}
        \centering
        \includegraphics[width=\textwidth, page = 1]{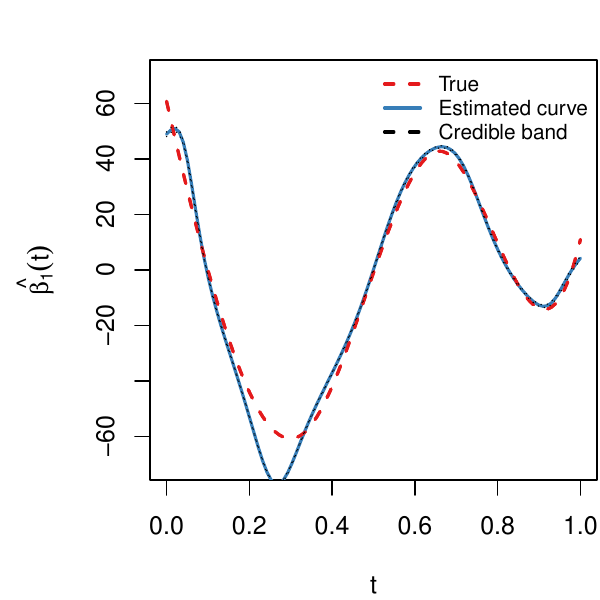}
        \caption{$\sigma^2 = 0.5$}
    \end{subfigure}
    \caption[Simulation Study 3. Estimated non-zero partial functional coefficient with credible bands when $n = 100$.]{Simulation Study 3. Estimated curves (blue) for the non-zero partial functional coefficient with corresponding 95\% credible bands for one of the simulated datasets under the scenario with sample size $n = 100$ and error variances $\sigma^2 = 0.1, 0.5$. The true partial non-zero functional coefficients is shown in red.}
    \label{fig:sim3_cred_n_100_sofr}
\end{figure}
